# Supplementary material for: PIANIST: Learning Partially Observable World Models with LLMs for Multi-Agent Decision Making
Source: arXiv:2411.15998 source file (2024-11-24)
Supplement: Supplementary file 1 [file ablation.tex]

\section{Other Ablation Studies}
\label{sec:ablation}

\subsubsection{Base LLM Model}
% How important is the base LLM for self-improvement? Would a bigger model perform better than a smaller one?
We show the performance of different base models in Figure \ref{fig_gpt_4_35}. 

\begin{figure}[h!]
    \centering
    \includegraphics[width=0.5\columnwidth]{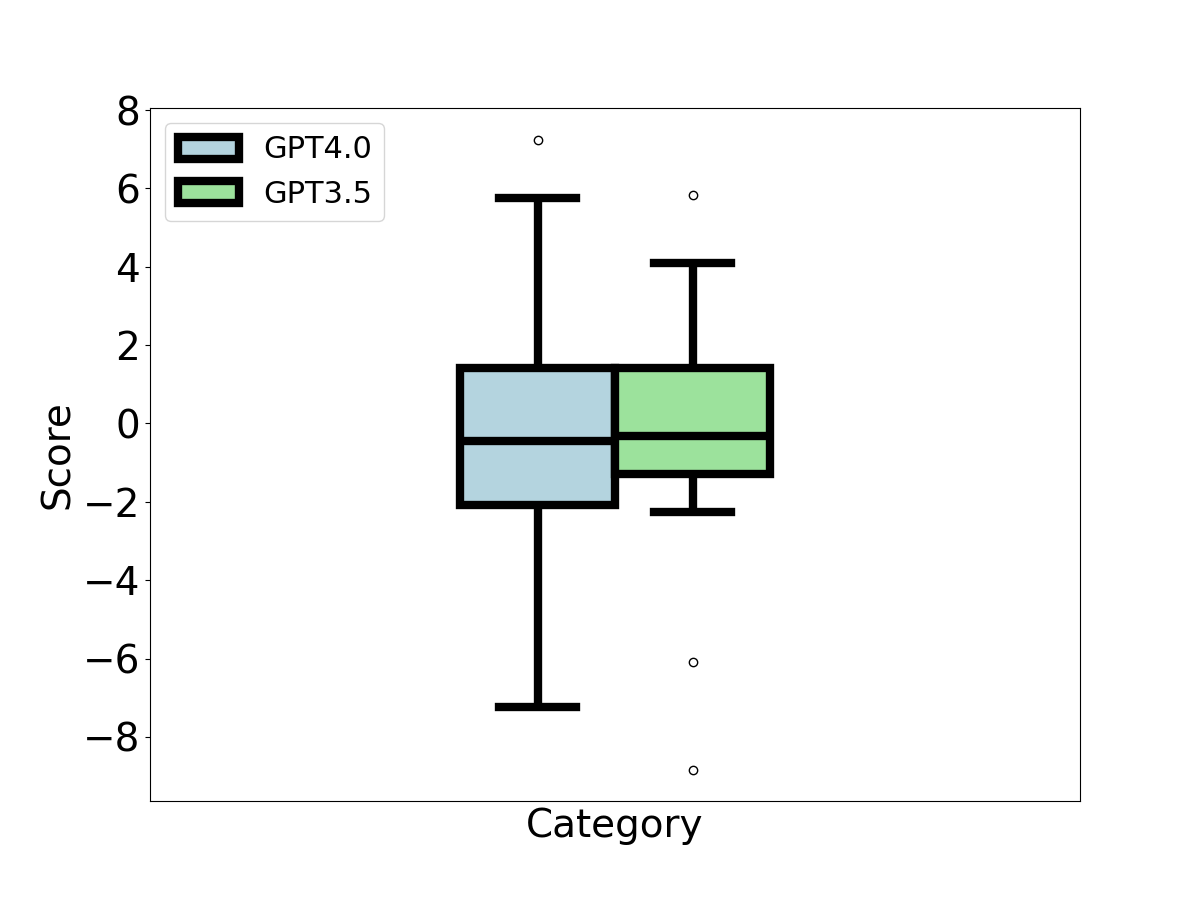}
    \caption{Game play performance of base LLM models on six card GOPS: GPT3.5 and GPT4.0. We see that the two language models perform similarly with our method.}
    \label{fig_gpt_4_35}
\end{figure}

\subsubsection{Search Budget}
How does the effectiveness of the search+LLM agent scale with regards to the search budget? Does having a larger search process help achieve better performance?

\begin{table}[ht]
\centering
\caption{Average score difference for MCTS (num\_rollout=32) + LLMFunction (Player1, top-3 functions shown in the table) vs. MCTS (num\_rollout=32) + RandomRollout (Player2, num\_rollout=10); 100 games for each experiment;}
\begin{tabular}{@{}ccccccc@{}}
\toprule
\multirow{2}{*}{budget} & \multicolumn{2}{c}{Best Func.} & \multicolumn{2}{c}{2nd Best Func.} & \multicolumn{2}{c}{3rd Best Func.} \\
                        & Player 1     & Player 2     & Player 1         & Player 2        & Player 1        & Player 2        \\ \midrule
16                      & -0.91           & 0.91           & -0.7             & 0.7            & -0.88            & 0.88            \\
32                      & -0.95           & 0.95           & 0.44             & -0.44            & -0.73            & 0.73            \\
64                      & -1.14           & 1.14           & 1.15           & -1.15           & 0.46            & -0.46            \\
128                      & -1.28           & 1.28           & 0.36           & -0.36           & 0.25            & -0.25            \\
256                     & -0.45           & 0.45           & -0.85           & 0.85           & -0.42            & 0.42            \\
inf                     & -1.5           & 1.5           & -2.26          & 2.26           & -1.03           & 1.03             \\ \bottomrule
\end{tabular}
\end{table}

% \subsubsection{Group evaluate vs. Benchmark evaluate}
% Are the intermediate performance estimators a good predictor of final performance?
% Does self-play help?

% \subsubsection{Feedback examples}
% Does more feedback examples provided to the LLM help the improvement process?

% \subsubsection{LLM temperature}
% Does having a higher temperature for the LLM (and thus more diversity in generations) improve self-improvement performance?
