# Supplementary material for: PIANIST: Learning Partially Observable World Models with LLMs for Multi-Agent Decision Making
Source: arXiv:2411.15998 source file (2024-11-24)
Supplement: Supplementary file 2 [file avalon_agent_implementation.tex]

\section{Avalon Agent Implementation Details}
\label{sec:avalon_agent}

We describe in detail how we implement our model below and as shown in figure \ref{fig:agentframework}. Unless otherwise specified, the word `action' will refer to non-dialogue actions. Note that we do not conduct search over raw dialogue space since that is not very computationally feasible. Instead, we search over intended actions and condition our dialogue on that. 

Specifically, the language component consists of a dialogue analyzer and a dialogue generator, while the moves component consist of the action planner. Whenever the agent needs to speak, they first analyze what was said so far in the current discussion round using the dialogue analyzer. The dialogue analyzer, with the help of an LLM, updates the internal beliefs of the agent. For example, in Avalon, internal beliefs might include the probability that the agent assigns to each other player of being Evil and of being Merlin. These beliefs are then passed to the action planner, which uses them to figure out the best next move, i.e. the action intent. The action intent is then passed to the dialogue generator, which generates dialogue with the help of an LLM. 
When the agent needs to take a move, we run through the same process except that the agent takes the action intent as the move and no dialogue is generated.

\begin{figure}
    \centering
    \includegraphics[width=1.1\textwidth]{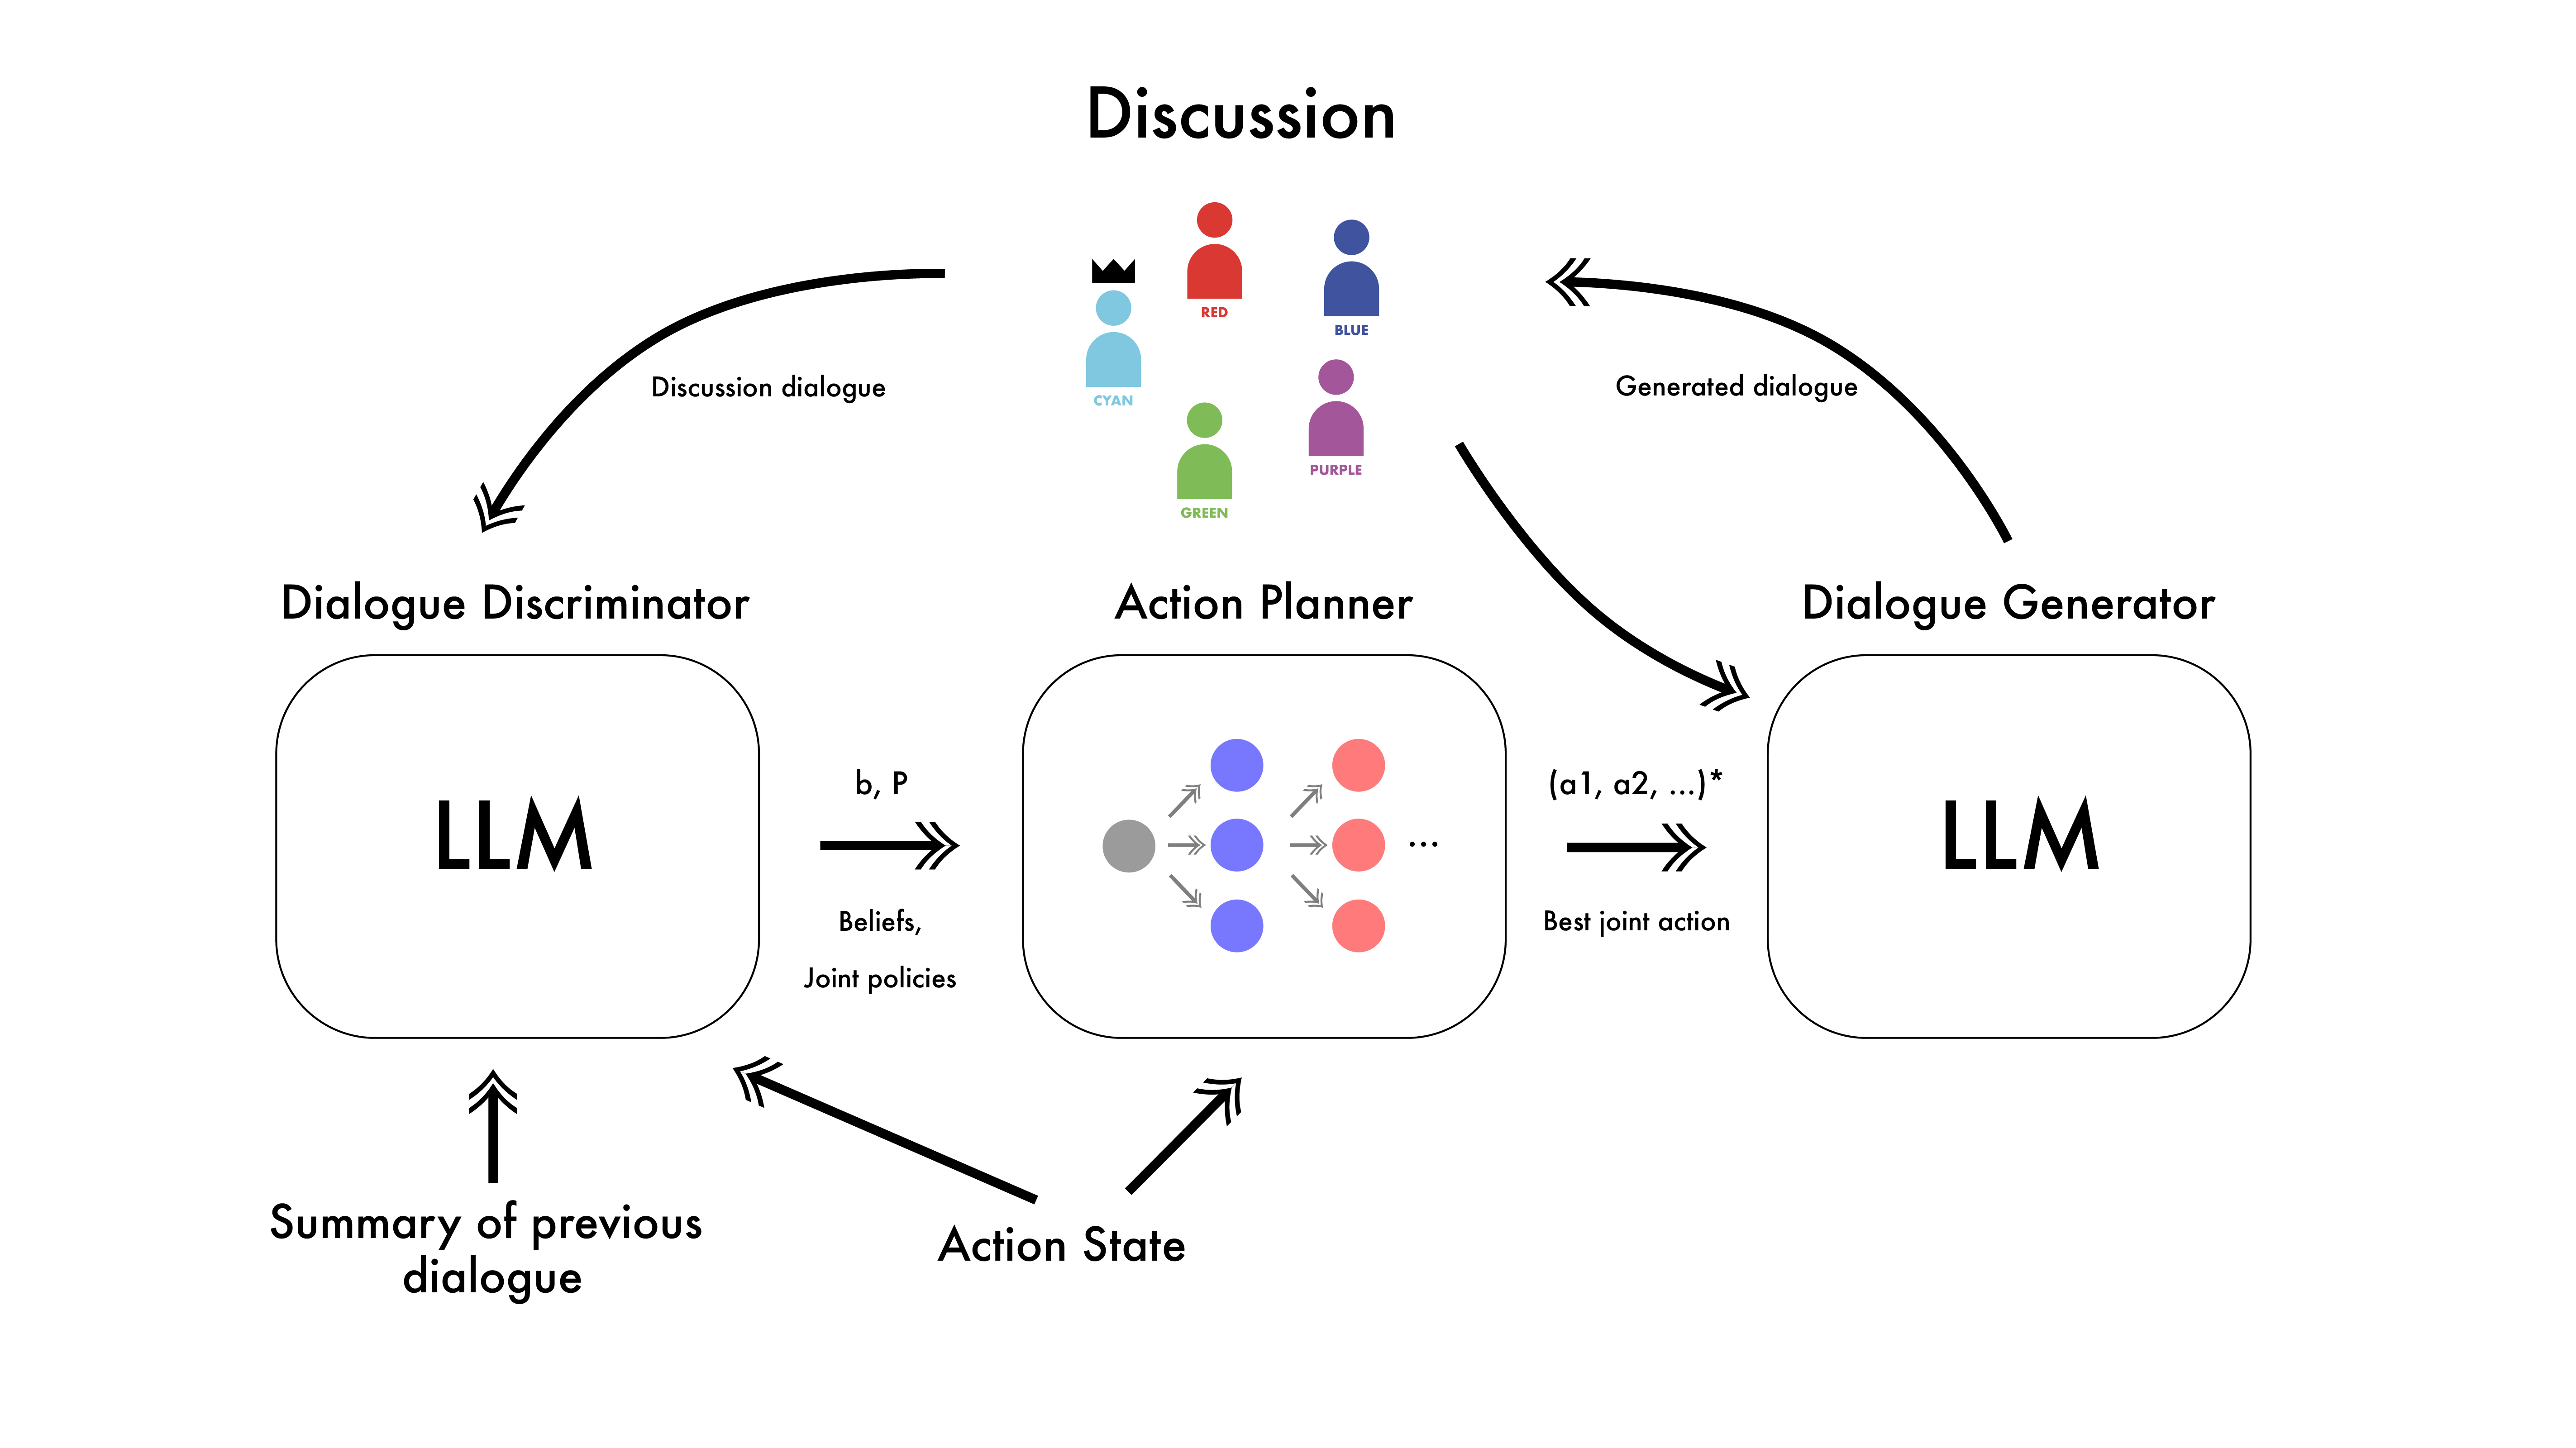}
    \caption{Overview of the LLM-powered agent, including the three main modules that we use to generate dialogue during discussion}
    \label{fig:agentframework}
\end{figure}

\subsection{Dialogue Analyzer (Discriminator)}
The dialogue analyzer $f_{ana}$ takes as input $\bs{I}$ information set (partial information) of the current state for the player, $\bs{d}_t$ the discussion so far this round, and $\bs{b}$ some prior beliefs about the hidden state of the game, and returns $\hat{\bs{b}}$, the updated beliefs, and $\hat{\bs{\Pi}}_t$, the predicted joint action policy of the all the players (i.e. the action intent) for the next action step $t$. Recall that simultaneous games can be expanded as partial information games, where the simultaneous moves are treated as hidden information. Hence, we are essentially predicting a distribution over the hidden states $\bs{s}$ given the information set $\bs{I}$ using the dialogue analyzer. 

\[\hat{\bs{b}}, \hat{\bs{\Pi}}_t = f_{ana}(\bs{I}, \bs{d}_t, \bs{b})\]

In the context of Avalon, $\bs{I}$ will contain information such as (1) the dialogue this round so far (2) summary of the dialogue from previous rounds (3) mission track record (4) historical record of actions taken by players in previous rounds, and (5) private information of the player such as who is Good and Evil. $\bs{b}$ will contain information on (1) the probability of each player being Evil and (2) the probability of each player being Merlin, both conditioned on the private information contained in $\bs{I}$. While a full treatment of the distribution over the hidden state space $\mathcal{S}$ we require assigning probabilities to each possible combination of Good and Evil players, not just assessing the marginal probability of each player being Good individually, in practice 

% or the probability of each possible combination of good and evil players in the game. either be

We implement $f_{ana}$ using an LLM, which is fed $\bs{I}$, $\bs{d}$, $\bs{b}$ (converted to natural language form) as prompts, along with some instruction prompt $\bs{\phi}_{ana}$ that prompts it to produce $\hat{\bs{b}}, \hat{\bs{\Pi}}_t$. Specifically, 

\[f_{ana}(\bs{I}, \bs{d}_t, \bs{b}) = f_{LLM}(\bs{\phi}_{dis}, \bs{I}, \bs{d}, \bs{b})\]

We show examples of such prompts in Appendix \ref{sec:dialogue_gen_anal}. 

% An example prompt that is fed to the LLM might be the following:\\

% \begin{tcolorbox}[title=Example Discriminator Prompt $\phi_{dis}$ ]
%   <$\bs{s}$> You are player 3, a servant of Arthur. The current state of the game is that the first mission succeeded and the second mission failed with one fail observed. Player 2 proposed the first mission with players 2 and 3 on it, and all players approved of the mission. Player 3 proposed the second mission with players 2,3,and 4 on it. Everybody except players 2 and 5 approved. 
%   <$\bs{s}$> 

%   <$\bs{d}$> In the discussion so far, player 1 said ``Player 3 obviously sabotaged the last mission''. Player 2 said ``I was with player 3 on the first mission, so I suspect player 4 more than player 3''.
%   <$\bs{d}$> 

%   <$\bs{b}$> You previously believed that the probability of player 1, 2, 4, and 5 being evil are 0.7, 0.3, 0.5, and 0.5 respectively. 
%   <$\bs{b}$>

%   <$\phi_{dis}$> What do you think the probability of each player being evil is now? What team do you think player 4 will choose, and which players do you think will vote to approve?<$\phi_{dis}$>
% \end{tcolorbox}

\subsection{Action Planner}

Given $\hat{\bs{b}}$ the belief prior, $\hat{\bs{\Pi}}_t$ the predicted joint action policy for all players, and $\bs{s}$ the representation of the current state, the action generation model $f_{act}$ generates a probability distribution over possible actions $\bs{\pi}^i$ for the main player $i$ that is the best response to $\hat{\bs{\Pi}}_t$. We do so by using search techniques to look ahead and find the best response. 

\[\bs{\pi}^i = f_{act}(\hat{\bs{b}}, \hat{\bs{\Pi}}_t, \bs{I})\]

More specifically, in our search implementation, at the first layer, we first sample across possible hidden states $\bs{s} \sim \hat{\bs{b}}$ according to the belief prior. At the second layer (i.e. the first action stage $t$), we calculate expected $q$-values for each action $a \in \mathcal{A}$ that the main player can take if the other players play actions $\bs{a} \sim \hat{\bs{\Pi}}_t$ according to the predicted joint distribution. In subsequent action stages, the search process will assume that other players play according to their policy simulated and induced by the value heuristic that is not dialogue dependent. We then take the best response action $a^*_i = \max(\bs{\pi}^i)$ as the intended action. Since this is a partial information game, expected $q$-values are taken across information sets, not states. We describe how our action planner is implemented in more detail in Appendix \ref{vh_implementation}.

% policy prior $\bar{\bs{\Pi}}_{>t}$
% \begin{figure}
%     \centering
%     \includegraphics[width=\textwidth]{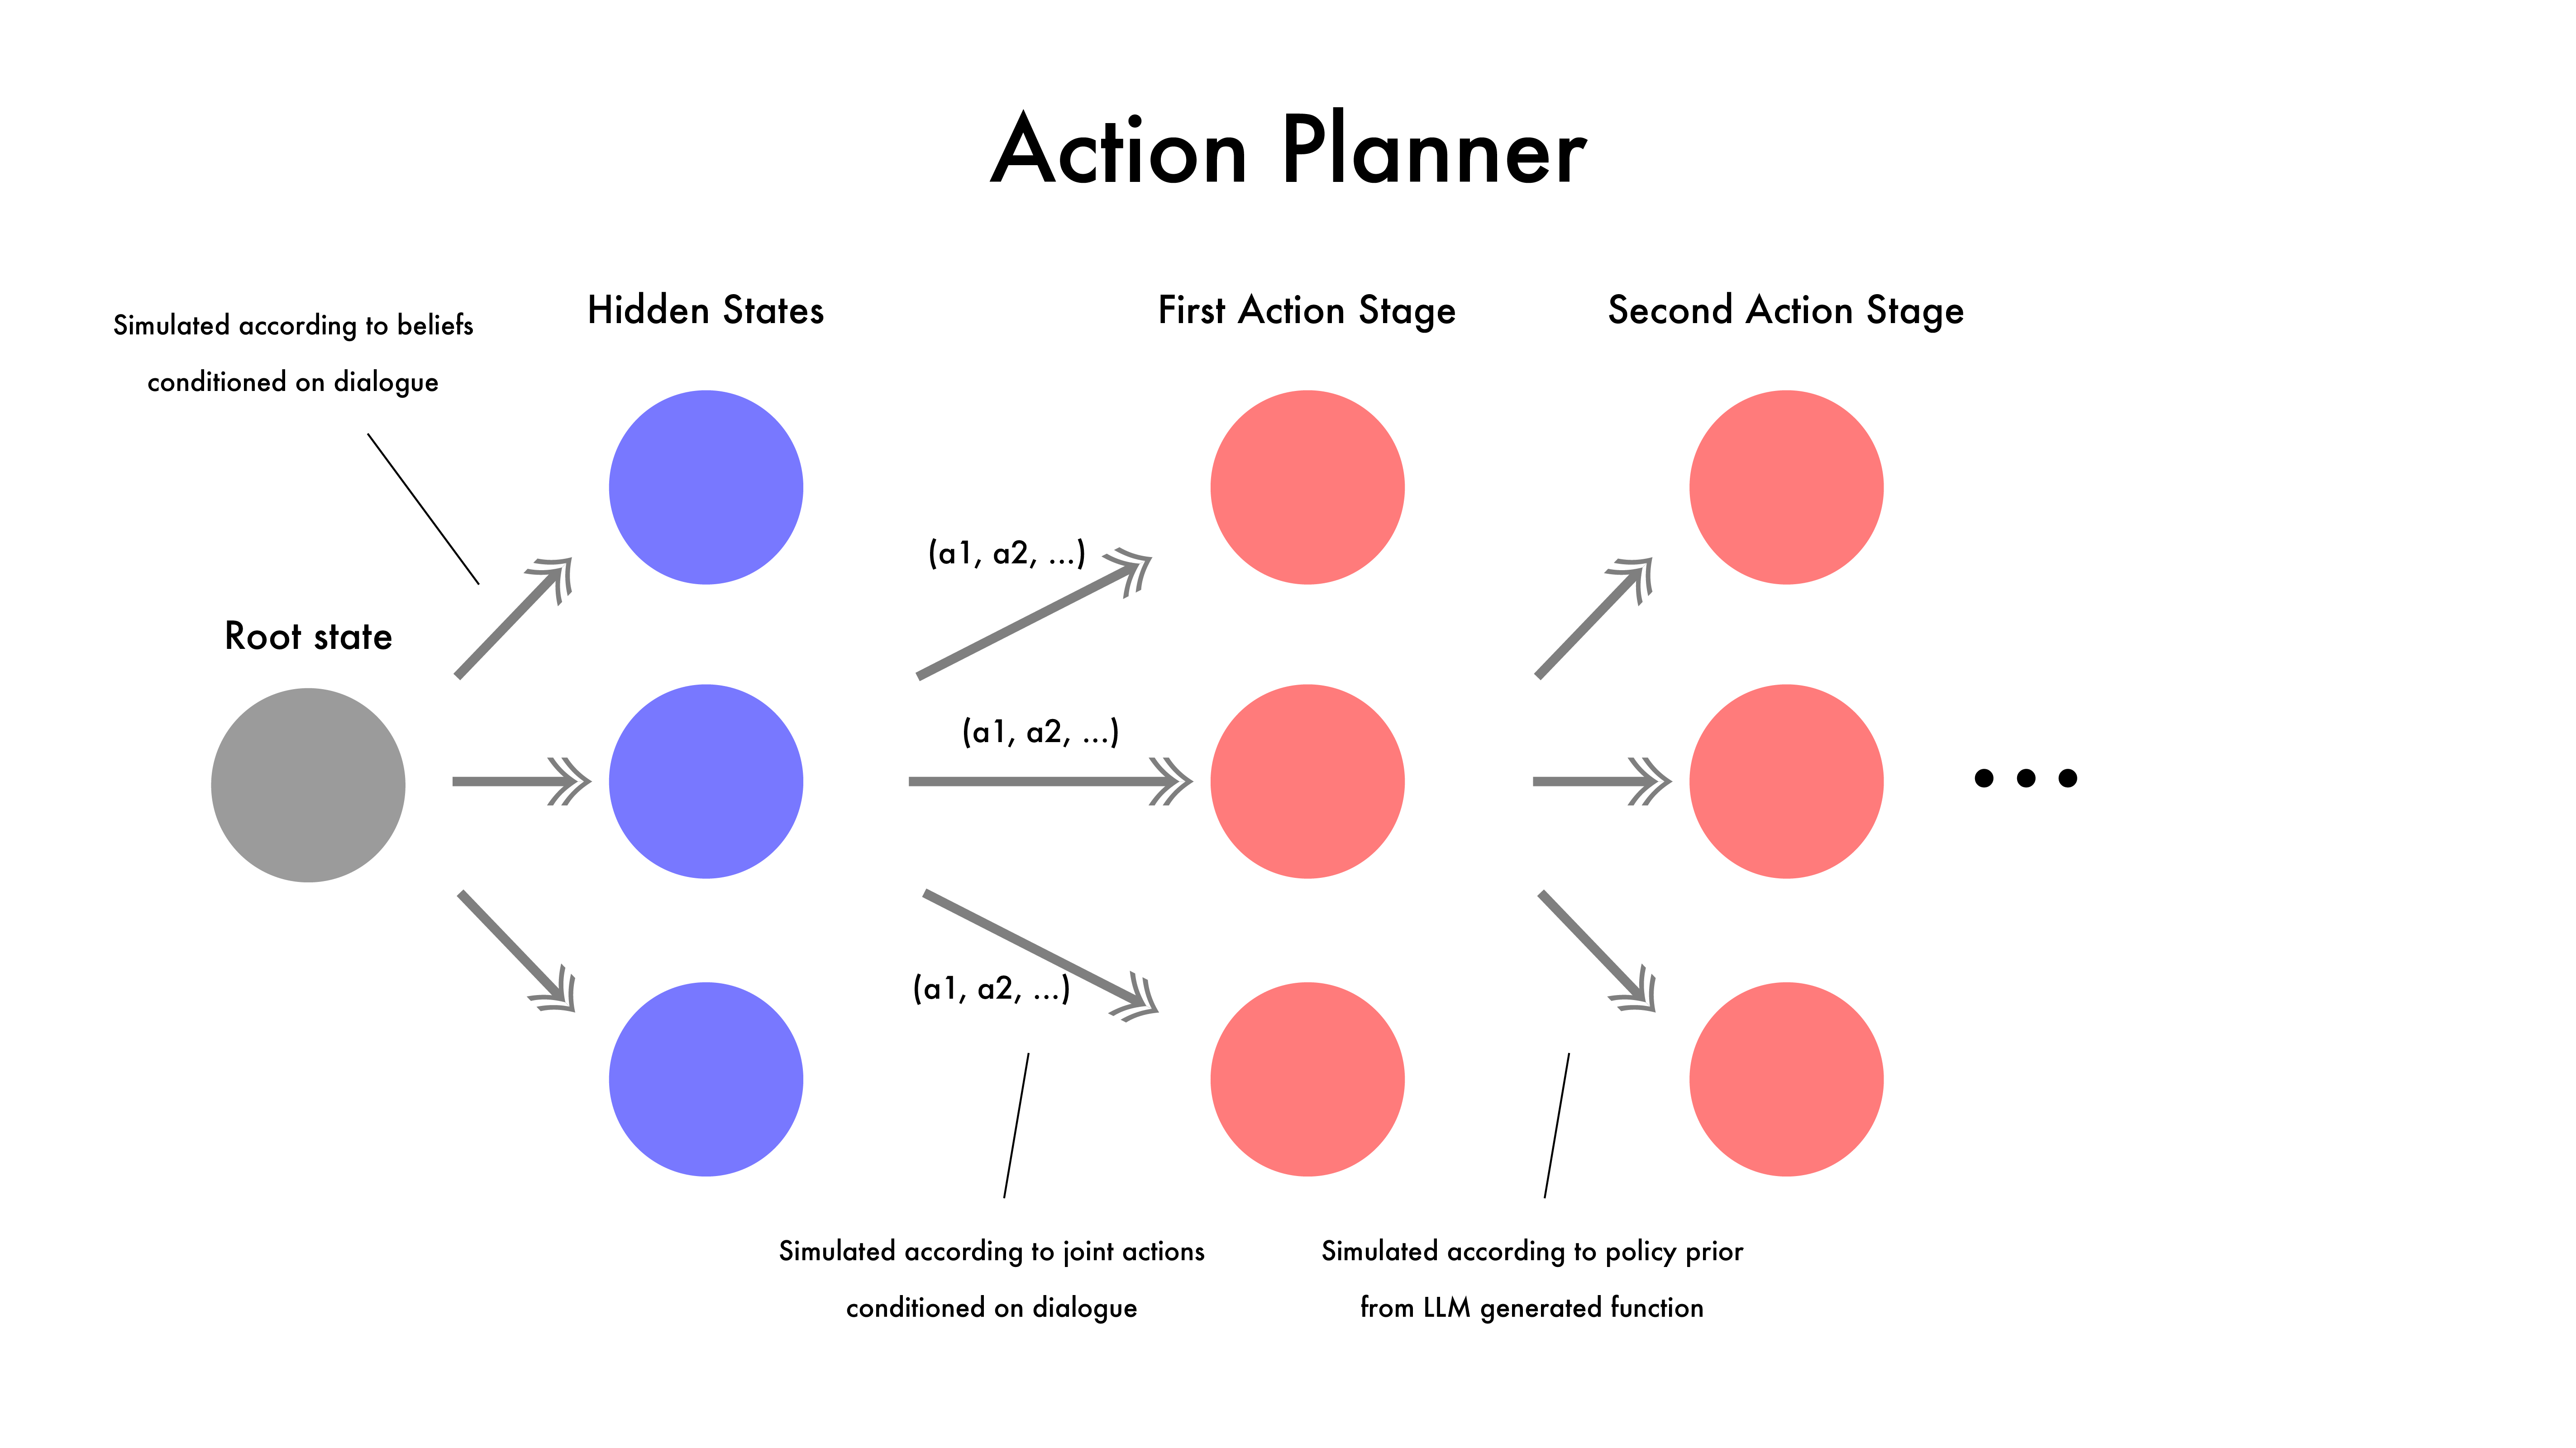}
%     \caption{Diagram of the action planner, where we use search techniques and information distilled from the dialogue discriminator to produce action intents}
%     \label{fig:actionplanner}
% \end{figure}

\subsection{Dialogue Generation}

The dialogue generator $f_{gen}$ takes as input $\bs{I}$ some representation of the current information set and $a^*_i$, the intended best response action, and outputs dialogue $d$.
\[d = f_{gen}(\bs{I}, a^*_i)\]
We will implement $f_{gen}$ using an LLM, which is fed $\bs{I}$ and $a^*_i$ directly as prompts, along with some instruction prompt $\phi_{gen}$ that prompts it to produce realistic sounding dialogue that helps it achieve its intended action. 

For example, perhaps the player wants to approve the next team. Then it should try to generated dialogue that convinces the other players to also approve. 

We show examples of such prompts in Appendix \ref{sec:dialogue_gen_anal}.
