# Supplementary material for: PIANIST: Learning Partially Observable World Models with LLMs for Multi-Agent Decision Making
Source: arXiv:2411.15998 source file (2024-11-24)
Supplement: Supplementary file 3 [file avalon_game.tex]

\section{Resistance: Avalon Game Description}
\label{sec:avalon_rules}
\begin{figure*}[h]
    \centering
    \includegraphics[width = 1\textwidth]{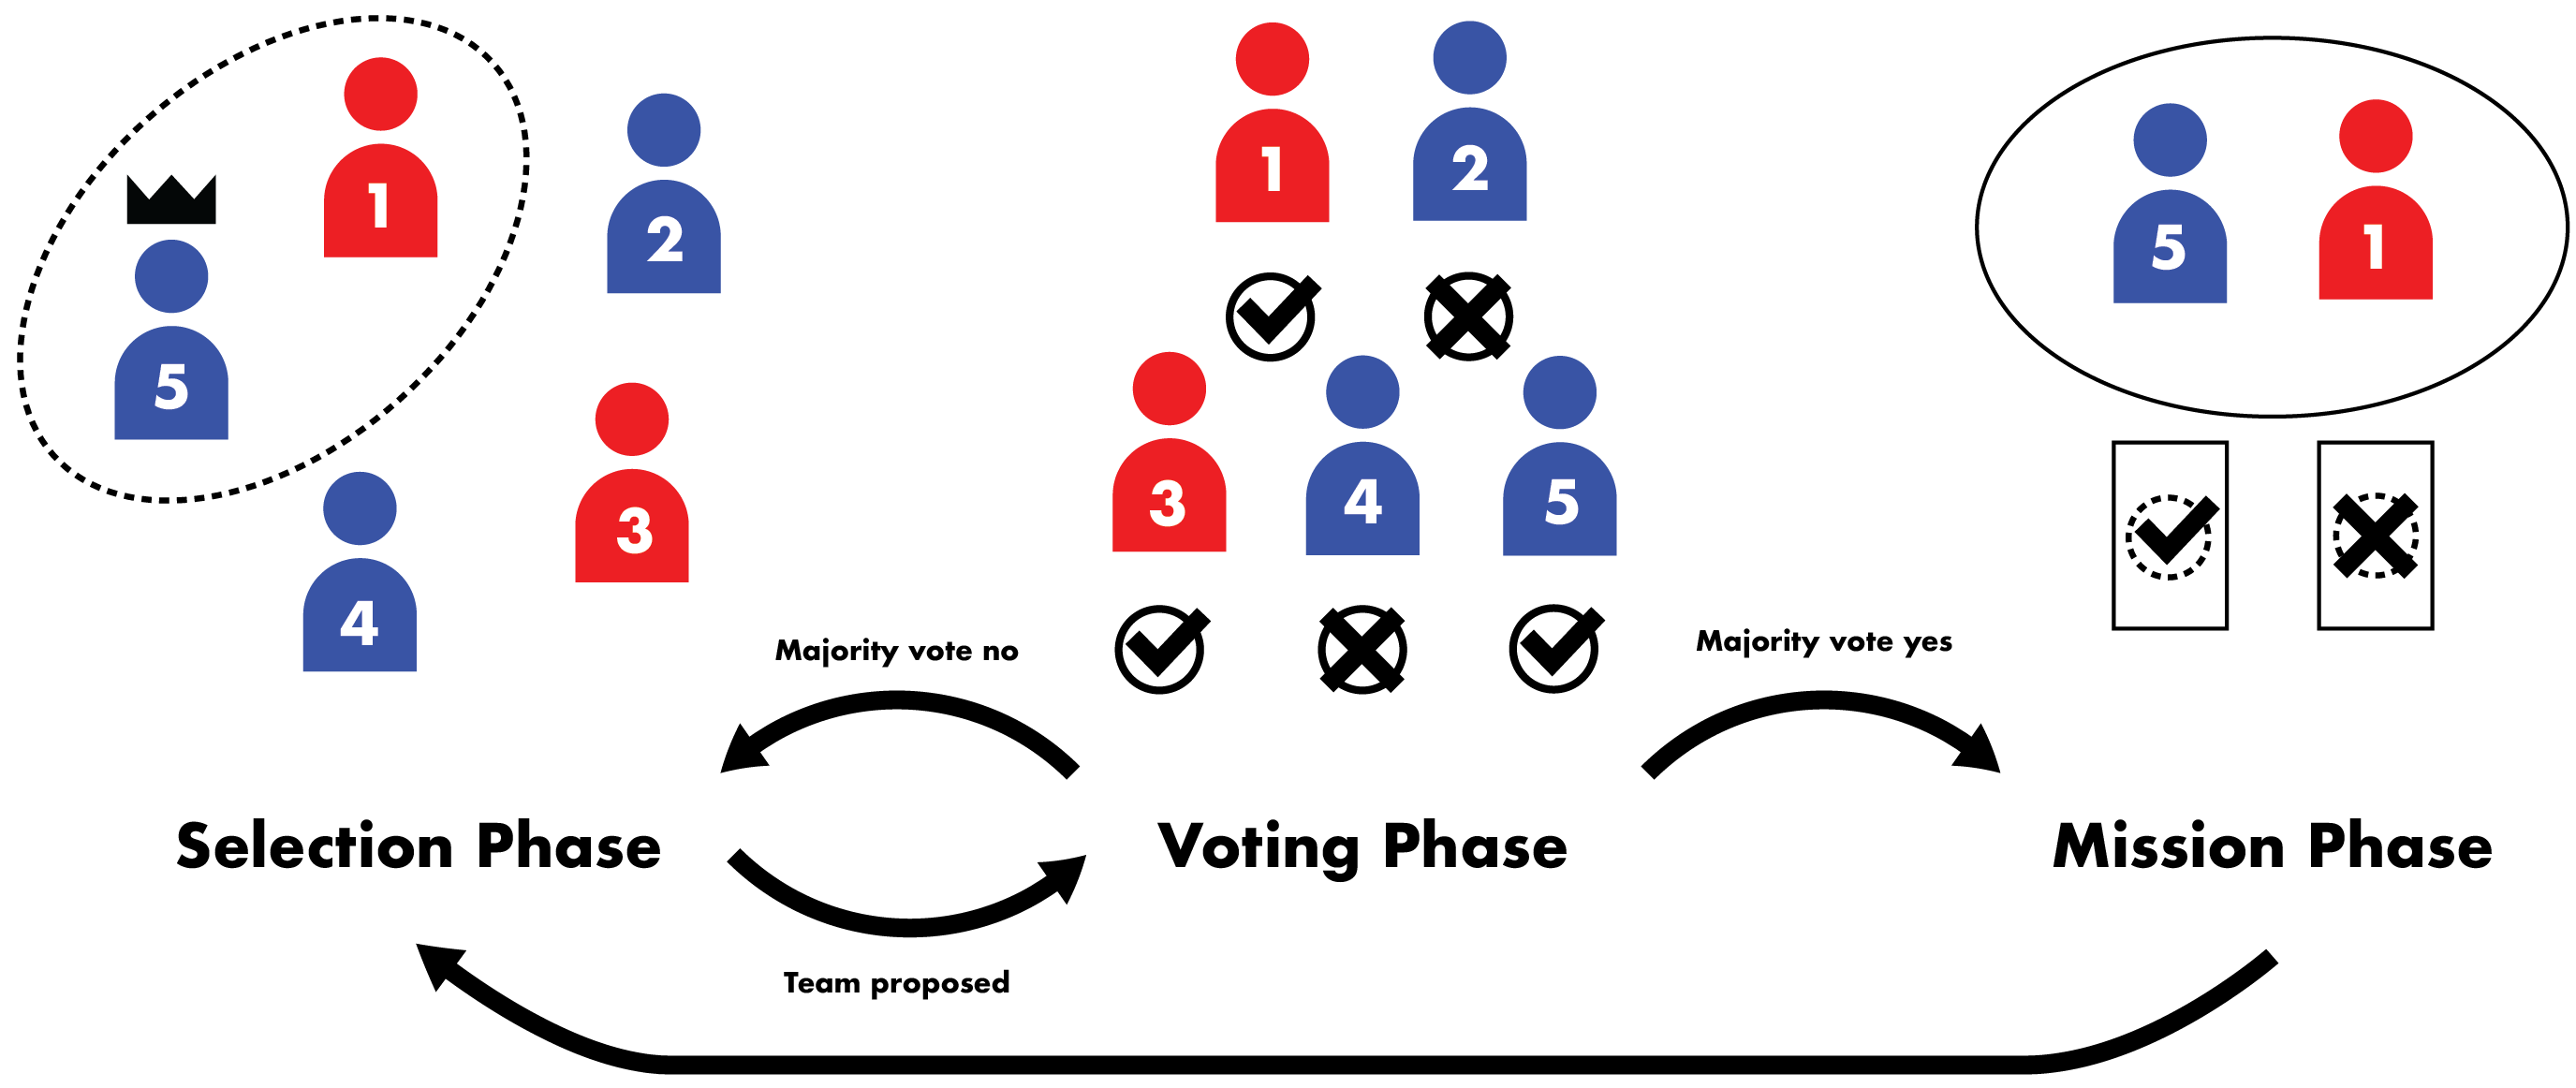}
    \caption{\textbf{The three phases per round of Resistance game}. Good players are shown in blue, while Evil players in red. In \textit{Selection Phase}, the team leader (player 5 in this round) proposes a team (player 1 and 5, himself). In \textit{Voting Phase}, all players vote publicly whether to approve this team or not. If the strict majority votes yes, the team is approved and moves on to the mission phase. Otherwise, redo the \textit{Selection Phase} with the next player as leader. If the team goes on the \textit{Mission Phase}, selected team members (player 1 and 5) anonymously vote to pass or fail the mission. If at least one person (player 1, as he is the evil player) votes fail, the mission fails. Otherwise, it succeeds.}
    \label{fig:phases}
\end{figure*}

\begin{figure*}[t!]
    \centering
    \includegraphics[width = 1\textwidth]{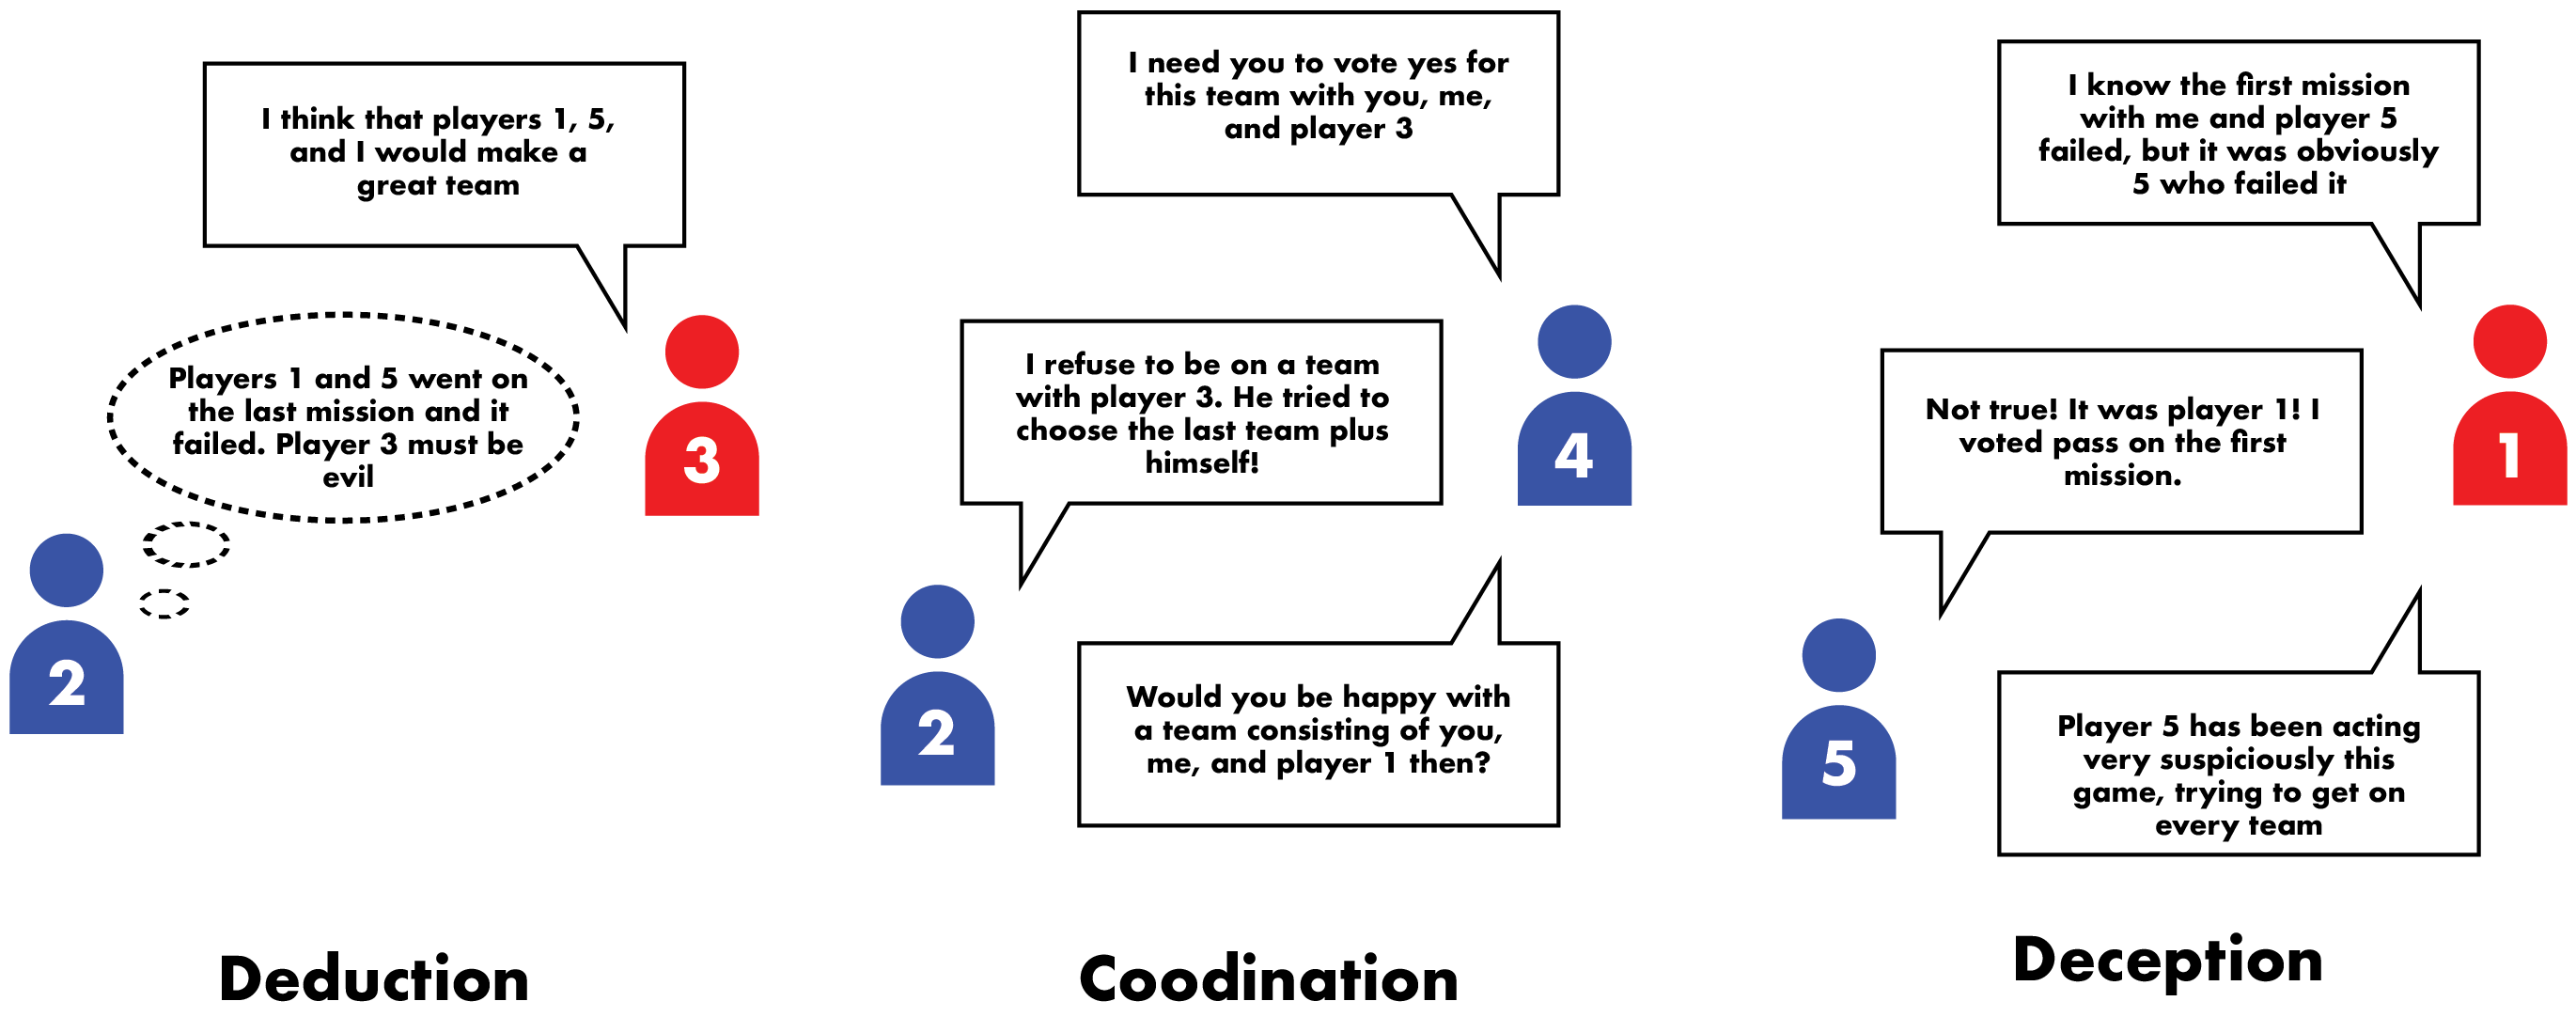}
    \caption{\textbf{Communication Skills required to play Avalon}. 1) First, they use logical reasoning to analyze the voting pattern and dialogue of other players and deduce their motives. 2) they must coordinate, communicate, and persuade their teammates to follow a particular strategy. 3) they must also hide their identity and motives through deception.}
    \label{fig:challenges}
\end{figure*}
We describe the game in more detail here. 
% In essence, Avalon is a game about sets of players, and selecting the right set of players to go on missions. 
There are four phases in the game where players need to make decisions: (1) \textbf{team selection phase}, (2) \textbf{voting phase}, (3) \textbf{quest phase}, and (4) \textbf{assassination phase}. The game alternates between the first three phases until the end condition is reached, at which point we move on to the assassination phase. Each phase also contains \textbf{discussion} where players can challenge others, defend themselves, and negotiate. A flowchart of the game is presented in Figure \ref{fig:flowchart}, and an Avalon Rule Prompt is included in Section \ref{box:avalon-rules-pt}.

\subsection{Roles}
There are four basic roles in Resistance Avalon: \textbf{Servant} of Arthur, \textbf{Minion} of Mordred, \textbf{Merlin}, and \textbf{Assassin}. The \textbf{Servant} is a basic good character who does not know the identity of any of the other players. The \textbf{Minion} is a base evil character who knows who is good and evil but does not know the specific roles of each player. \textbf{Merlin} is a unique good character who knows who is good and evil. The \textbf{Assassin} is a unique evil character who knows who is good and evil, and in addition, has the ability to assassinate a character at the end of the game. If that character is \textbf{Merlin}, the evil team wins.

% Though the assassin has final say on who to assassinate, they are encouraged to consult their peers before doing so. 

Good players will always outnumber evil players.
% , no matter the number of players. 
Hence, evil players must pretend to be good in order to be voted in on teams (and thus sabotage missions). \textsc{Servant}s will thus need to sniff out the evil players through their actions and dialogue. \textsc{Merlin} is usually the only good player with additional information, so they will need to discreetly guide the \textsc{Servant}s in the right direction. Servants also need to protect \textsc{Merlin}, so a common strategy is for \textsc{Servant}s to pretend to have hidden information so that evil players will think that they are \textsc{Merlin}. Evil players will be trying to sniff out \textsc{Merlin} at the same time, so deduction skills are required for all roles. 

\subsection{Actions for each Phase}
Depending on the phase \textbf{team selection}, \textbf{voting}, \textbf{quest}, and \textbf{assassination}, players may conduct different actions. We detail the specific actions that players can take in each of these phases below. 

During the \textbf{team selection phase}, only the current \emph{leader} has to make a choice. Leadership passes around the players sequentially in a loop. The action space of \textbf{team selection} for the leader consists of all subsets of the players with size equal to the mission team size. The mission team size is different for each mission and is determined by the total number of players in the game. For example, in a 5-player game, on mission No.4, the mission team size is $3$, so any subset of $\{1,2,3,4,5\}$ with size $3$ would be a valid action. After the team proposal is determined by the leader, we move on to the \textbf{voting phase} with the selected players. 

During the \textbf{voting phase}, \emph{every} player in the game needs to simultaneously vote either \textsc{Approve (1)} or \textsc{Reject (0)}. Votes are publicly revealed to all players, so players can see what other players voted. If a strict majority votes \textsc{APPROVE (1)}, we then move on to the quest phase with the team that was approved. Otherwise, we move back to the selection phase. Note that if four teams have been rejected in a row, and this is the fifth time a team is proposed (for the same mission), we skip the voting and move directly to the \textbf{quest phase}. This prevents the game from dragging on forever.
% \footnote{Technically, in the official rules, the mission fails if the fifth team is rejected. However, since approving the fifth mission is the dominant strategy for all good players, the fifth mission will always be approved in either case}

During the \textbf{quest phase}, \emph{each selected player on the approved team} votes anonymously to either \textsc{Pass (1)} or \textsc{Fail (0)} the mission. The number of votes of \textsc{Pass} vs \textsc{Fail} are then revealed to everybody. If the number of \textsc{Fail}s is greater than or equal to the number of \textsc{Fail}s required for the mission to fail (usually 1), then this mission is marked as a failure. 
% The number of fails required is different depending on how many players and which mission we are on. 
Otherwise, this mission is marked as a success. Hence, good players usually have no incentive to fail missions, while evil players will want to have enough failures to pass the failure threshold. If three out of five missions fail, evil wins immediately. Otherwise, if three out of five missions succeed, we move on to the assassination phase. 
% Hence, there is no need to continue the game once we see three failed or successful missions. 

% When the number of successful missions or number of unsuccessful missions hits 3, we enter the $assassination$ phase. 

\begin{figure*}[t!]
    \centering
    \includegraphics[width=1\textwidth]{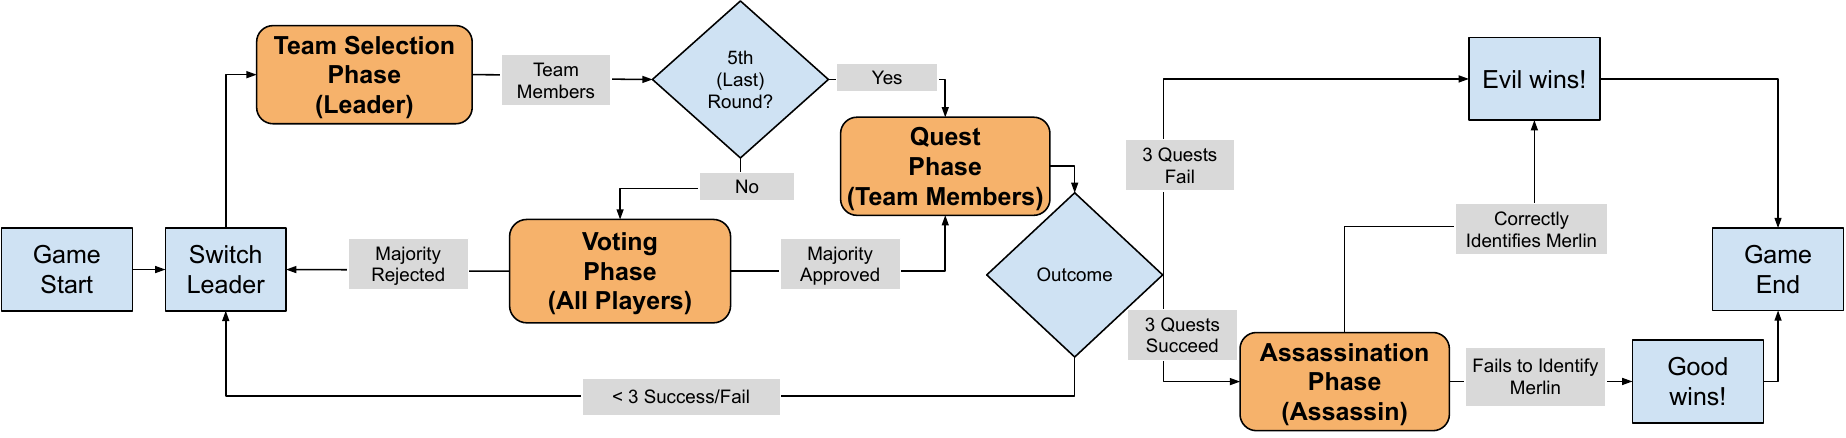}
    \caption{\textbf{Flowchart illustrating the various game states and transition diagram}. Round boxes indicate game states (phases) where the player (role highlighted in bracket) has to make decisions}
    \label{fig:flowchart}
\end{figure*}

\subsection{Discussion}
Group discussion occurs between the \textbf{quest} and \textbf{selection} phases, as well as right before the \textbf{assassination} phase. Players may not communicate during any other time. All conversations are public, and there is no private communication. Typically players may discuss in any format of their choosing as long as only one person is speaking at a time. Some examples of formats include a natural (spontaneous) seminar style (most common, where there is no fixed order of speaking), or sequentially (where players speak in some predefined order). Interruptions and arguments between two players are very common between human players. 
% Typically there is a time limit on how much \textbf{discussion phase} can occur before we move on to the voting phase to make sure the game keeps moving. 

Usually, players will spend this time discussing a couple of key topics, including (1) the \textbf{observations} they made, (2) the \textit{guessed identities and sides} of players, and (3) the \textbf{plan} for the next mission. The team leader will usually spend this time asking for advice on what team to select and gathering support for that team. Persuasion and adhering to the preferences of other players are usually key to getting a team approved. Players can also accuse other players of being evil, though arguments will need to be justified in order to be persuasive. 

% As an example in Figure~\ref{fig:challenges}
For example, a player (player 3) could start off by stating their (1) \textbf{observations} of what happened in the previous mission. One \textsc{Fail} was observed, so at least one player on the previous team (consisting of players (1,2,3)) is evil. Player 3 then emphasizes that both Players 1 and 2 voted \textsc{Approve} for the previous mission, which ended up a failure. Moreover, the team was proposed by Player 1 in the first place. Player 3 then moves on to discuss the (2) \textbf{identities} of other players. The player says that, despite the fact that only one \textsc{Fail} was observed, both Players 1 and 2 are evil since they both voted to \textsc{Approve} previously. Player 0 is probably good since they voted to \textsc{Reject} in the previous mission, and Player 3 is also good since they also voted to \textsc{Reject}, even though they were on the mission. Player 3 then says what they think the (3) \textbf{plan} should be. Specifically, Player 3 says that they should reject the current team no matter what since Player 2 is the leader and is evil. The leadership will then pass to Player 3, who will choose the team $(0,3,4)$, which good players should vote to approve since it does not contain any suspected evil players\footnote{At this point, Player $2$ reveals that they are the assassin and assassinates Player $3$, who is indeed \textsc{Merlin}. Player $3$'s intuition and analysis were way too correct to be a \textsc{Servant}}.

\subsection{Game Ending and Assassination}
In classic \textsc{Resistance}, a good team wins immediately if three missions are successful. In \textsc{Resistance Avalon}, there is an additional assassination phase if three missions are successful. 
During the \textbf{assassination} phase, the \textsc{Assassin} player chooses one player to assassinate. If that player is \textsc{Merlin}, then evil wins. Otherwise good wins. 

Before they assassinate a player, the \textsc{Assassin} player can and is encouraged to discuss with the other players (mostly their teammates). good players are also welcome to join in on this discussion to mislead the evil players, though it rarely helps. Players can discuss in a format of their choosing, though there is usually a time limit on how long players can discuss before reaching a decision.

\begin{tcolorbox}[title=Avalon rules prompt,  colframe=custom3] \label{box:avalon-rules-pt}
The game you are interested in is called The Resistance: Avalon. The Resistance: Avalon is the game of hidden identities and social deduction. There are two teams in the game: Good and Evil. Each player has a hidden identity (role) and side. \\

There are five Quests in the game and five turns, one for each quest. Good players aim to help three Quests succeed, while Evil players aim to fail three Quests. Different quests require different numbers of players to participate. \\

At the beginning of the game, each player is assigned a role secretly and randomly. Private information is then revealed to each player. A random player is selected as the leader for the first round.\\

Each round, after a round of discussion, the leader will select a team of players to participate in the Quest. Then, all players will vote on whether to approve or reject the team publicly. If the team is approved (a strict majority vote to approve), the Quest will be carried out. If the team is not approved, the next player becomes the leader and the next round will start. If four teams are rejected in a row, the fifth team will automatically be approved.\\

If the team is approved, each team member chooses to pass or fail the Quest anonymously. Usually, if there is at least one failed vote, the Quest fails. Otherwise, the Quest succeeds. In either case, we move on to the next turn and the next quest. \\

Below are the roles in the game:

Servant of Arthur (Servant): A Good player who does not know who is on the Evil side. The Servant's job is to make sure that the three Quests succeed.

Minion of Mordred (Minion): An Evil player who knows who is on the Evil side. Minion's job is to fail three Quests without being identified by the Good players.

Merlin: A Good player who knows who is on the Evil side. Merlin's job is to make sure that the three Quests succeed without revealing themself to Evil.

Assassin: An Evil player who knows who is on the Evil side. Assassin's job is to assassinate Merlin if the Evil players can identify who Merlin is. If the Assassin successfully assassinates Merlin, the Evil players win the game immediately, even if three quests succeed.

Hence, Evil players usually know who is on the Evil side, but Good players usually do not know who is on the Evil side. \\

Players may make any claims during the game, at any point in the game. Discussion, deception, accusation, persuasion, and logical deduction are all equally important in order for Good to prevail or Evil to rule the day. Hence, players should rarely reveal their true identity to other players. Players will, can, and should lie to achieve their goals.\\
\end{tcolorbox}
