# Supplementary material for: PIANIST: Learning Partially Observable World Models with LLMs for Multi-Agent Decision Making
Source: arXiv:2411.15998 source file (2024-11-24)
Supplement: Supplementary file 4 [file baseline_improvement_methods.tex]

\section{Improvement method baselines}
\label{sec:improvement_methods}

\textbf{Line search} always reflects and improves upon the latest improved strategy. In other words, we implement a strategy, collect feedback from the environment on the strategy, then improve it using the LLM, rinse and repeat, in Reflexion style ~\citep{madaan2024self}.\\

\textbf{Greedy search} selects the best strategy from the last generation of improved strategies to improve upon each improvement cycle. Each improvement cycle, we take the best strategy from the previous improvement cycle and create $n$ different improved versions of it. We then collect feedback from the environment on these $n$ new strategies, and pick the best one to progress to the next improvement cycle. This is how Eureka ~\citep{ma2023eureka} improves reward functions using LLMs, similar to an evolutionary algorithm

\textbf{Best first search} improves upon the $k$ best strategies generated in any iteration of each improvement cycle, similar to beam search. However, unlike beam search, we can set the branching factor to greater than one, where we generate more than one strategy from each previous strategy selected. Tree of thought explored a similar approach for self improvement ~\citep{yao2024tree}.

\textbf{Best first search with thought} asks the LLM to improve upon the thoughts used to generate the $k$ best strategies before improving the strategy itself while conducting best first search. This is similar to adding a React style thought and action to the improvement step ~\citep{yao2022react}. 

\method is our method that uses an additional idea queue $Q$ 
and an idea generation step to guide the improvement process.  

All methods were run with the same budget, i.e. generating the same number of improved strategies, in our experiments where we compared the methods.
