# Supplementary material for: PIANIST: Learning Partially Observable World Models with LLMs for Multi-Agent Decision Making
Source: arXiv:2411.15998 source file (2024-11-24)
Supplement: Supplementary file 5 [file dialogue_examples.tex]

\section{Dialogue Guide LLM Prompt and Output Examples}
This sections shows the system prompts of dialogue guidance on LLM and several examples, including system prompts, idea generation prompts, and strategy implementation examples.

\subsection{System Prompts}
Below is the Dialogue guide system prompt.

\begin{tcolorbox}[title=Dialogue guide system prompt,  colframe=custom3, colback=white,]
You are a coach trying to write a section of a strategy guide on how to play a game well. \\
        
The specific section of the strategy guide you are writing right now is on how to play the Merlin role effectively during the discussion phase so that they can win the game. Recall that players often use the discussion phase to (1) gather information about other players, (2) try to convince other players of their innocence or guilt, and (3) try to persuade other players of a particular course of action.
The game you are interested in is called The Resistance: Avalon. The Resistance: Avalon is the game of hidden identities and social deduction. There are two teams in the game: Good and Evil. Each player has a hidden identity (role) and side. 
\end{tcolorbox}

Dialogue guide signature follows, specifying the structures and contents dialogues regarding role playing the Merlin.
\begin{tcolorbox}[colback=white,colframe=custom3,title=Dialogue guide signature]

Your guide should be in the form of a worksheet that the student can use to build their speech. You should order the worksheet questions in a way that makes logical sense, and you should have no more than six questions. Your questions should instruct the reader to write parts of their speech. \\

The title of your section should be ``Questions to fill out before speaking as the Merlin role''. Below is an example of how your worksheet should look like: \\

\begin{enumerate}

\item Questions to fill out before speaking as the Merlin role

\item Q1: Which player seems the most suspicious of you and why?

\item Q2: For the player that seems the most suspicious of you, produce a statement addressing their suspicious.

\item Q3: Which player is the quest leader?

\item Q4: Produce a statement addressing the quest leader to convince them to support your intended course of action/ desired team.

\item Q5: Which player is the most supportive of you?

\item Q6: Produce a statement addressing the supportive player to convince them to support your intended course of action/ desired team.

\end{enumerate}

\end{tcolorbox}

\begin{tcolorbox}[title=Example Generated Dialogue Strategy Guide for Assassin, colframe=custom3, colback=white]
\begin{enumerate}
\item Q1: Which player seems to have a deeper understanding of the game flow than normal Servants should possess?

\item Q2: Develop a non-confrontational statement to subtly challenge this player. This should cause them to either prove their innocence or reveal more clues about their identity.

\item Q3: Who has been the most influential in the team selection and voting process?

\item Q4: Devise a statement to express agreement with this player's viewpoint subtly. This should make you less suspicious while enabling you to manipulate the discussion.

\item Q5: Which player seems the most supportive of your views and actions in the game?

\item Q6: Craft a statement subtly emphasizing your alignment with this supportive player’s thoughts. This should increase your chances of being included in quest teams and reduce suspicion around you.
\end{enumerate}
\end{tcolorbox}

\subsection{Idea Generation Examples}

The following is the selected dialouge guide speaking as the Merlin role.
\begin{tcolorbox}[colframe=black, title=Select dialogue guide, colback=white]
Questions to fill out before speaking as the Merlin role
\begin{enumerate}
\item Who are the players you suspect are on the Evil side and why? \
\item Draft a subtle statement that casts doubt on these players without directly accusing them. \
\item Who is the current round leader and which players are you considering to suggest for the team? \
\item Create a subtle suggestion that influences the leader's team decision towards your preferred team without revealing your knowledge. \
\item What are the voting patterns you've observed and what do these patterns indicate about the players' identities? \
\item Analyze the voting patterns and team compositions proposed by each player to identify potential alliances or suspicious behaviors. Craft a statement to subtly address these observations without revealing your role. \
\item Which player seems the most supportive of Good and how can you align with them during the discussion phase to better ensure success for your team? \
\end{enumerate}
\end{tcolorbox}

A feedback example is provided for better understanding of dialogue guidance to teach LLM how to role play Merlin.
\begin{tcolorbox}[colframe=black, title=Feedback example description, colback=white]
Example 2: \\

The student using your guide was playing as player 0 in this example filled out your guide as follows:

\begin{enumerate}

\item Q1: Based on the statements made so far, I suspect Players 2 and 4 are on the Evil side. Player 2's suggestion of a team consisting of Player 1 and Player 2 seems too convenient, possibly indicating a desire to control the team composition. Player 4's agreement with Player 1 and Player 2 without offering any alternative team suggestions raises suspicion as well.

\item Q2: "I can't help but wonder if some players are trying to steer the team selection process in a particular direction. It's important for us to carefully consider all perspectives and not be swayed by potentially self-serving suggestions."

\item Q3: The current round leader is Player 1. I would suggest a team consisting of Player 0 (Merlin) and Player 1, as this would allow me to closely observe the actions of the other players and potentially guide the team towards success.

\item Q4: "Player 1, I believe that a team comprised of Player 0 and Player 1 would provide a strong foundation for success. By working closely together, we can ensure that our mission is carried out effectively."

\item Q5: The voting patterns so far show agreement among Players 1, 2, and 4, indicating a potential alliance or shared goals. Player 3's suggestion of including themselves in the team may also indicate a desire to control the outcome of the quest.

\item Q6: "I've noticed a pattern of agreement among certain players in the team selection process. It's important for us to consider all perspectives and not be swayed by potentially biased suggestions. Let's focus on working together as a team to achieve our common goal."

\item Q7: Player 1 seems the most supportive of Good based on their consistent emphasis on unity and success for the Quests. I will align with Player 1 during the discussion phase to ensure that our team is selected and the quest is completed successfully.

\end{enumerate}

Then they said the following during the discussion phase:\\

"Fellow players, as we embark on this quest, it is crucial that we approach the team selection process with caution and consideration. I have noticed a pattern of agreement among certain players, which could potentially indicate a desire to steer the outcome in a particular direction. It is important for us to carefully consider all perspectives and not be swayed by potentially biased suggestions.\\

I believe that a team comprised of Player 0 and Player 1 would provide a strong foundation for success. By working closely together, we can ensure that our mission is carried out effectively. Player 1 has consistently emphasized unity and success for the Quests, making them a trustworthy ally in this endeavor.\\

Let us focus on working together as a team to achieve our common goal, rather than allowing personal agendas to influence our decisions. Let us approach this quest with unity and determination, ensuring that Good prevails in the end. Thank you for your attention."
\end{tcolorbox}

% title=Feedback example description (continued)
\begin{tcolorbox}[colframe=black, colback=white]
Below is some feedback from the other players on how player 0 performed during the discussion phase. Recall that Good players are trying to access which other players are likely to be Good, while Evil players are trying to access which Good player is likely to be Merlin.\\

Player 3 with role Servant had the following thoughts on this discussion round: \\ 

Thought: 

Player 1's speech emphasizes unity and success for the Quests, which aligns with the goals of Good and decreases the probability of Player 1 being Evil. Player 2's statement also focuses on unity and careful consideration, indicating a commitment to the success of Good and decreasing the probability of Player 2 being Evil. Player 3's response as a Servant of Arthur is focused on the success of the Quests and unity, which aligns with the goals of Good and decreases the probability of Player 3 being Evil. Player 4's speech seems overly enthusiastic and focused on unity and cooperation, which could be a tactic to divert attention from their true identity as an Evil player. This raises suspicion and increases the probability of Player 4 being Evil. \\

Dictionary: 
\{0: (-1, 'decreased slightly'), 1: (-1, 'decreased slightly'), 2: (0, 'stayed the same'), 3: (-2, 'decreased significantly'), 4: (2, 'increased significantly')\}\\

Player 4 with role Assassin had the following thoughts on this discussion round: \\

 Thought:

Player 2 seems to suspect the Evil players (Player 3 and Player 4) without any evidence and is trying to steer the conversation towards them. This aligns with the behavior of Merlin, who knows the identity of the Evil players and is trying to subtly guide the Good players towards the correct decisions. This increases the probability of Player 2 being Merlin. On the other hand, Player 3's speech seems generally clueless and lacks any strategic insight, which decreases the probability of Player 3 being Merlin.\\

Dictionary:
\{0: (0, 'stayed the same'), 1: (0, 'stayed the same'), 2: (2, 'increased significantly'), 3: (-2, 'decreased significantly'), 4: (-2, 'decreased significantly')\}

\end{tcolorbox}

This is the prompt for feedback reflections.
\begin{tcolorbox}[colframe=custom5, colback=white, title=Prompt for feedback reflections]
\texttt{<System prompt>}\\
\texttt{<Game rules>}\\
You previously generated the following section of the strategy guide: 
\texttt{<Previous guide>}\\
Below is some feedback on how your guide performed when a student used it to play the game: 

\texttt{<Feedback examples>}\\
Based on the feedback given and the guide section you generated previously, what are some conclusions you can draw from the feedback? Make sure to cite the specific examples in the feedback to justify your analysis.
 \end{tcolorbox}

The following are the feedback reflections generated by LLM.
 \begin{tcolorbox}[colback=white,colframe=custom4,title=Generated feedback reflections]

In Example 0, Player 0 effectively followed the guide by suspecting certain players of being on the Evil side, crafting subtle statements to cast doubt on them, and aligning with players supportive of Good. This led to Player 0 being perceived positively by other players, with Player 2's probability of being Merlin decreasing significantly due to their behavior aligning more with the Evil side. \\

In Example 1, Player 0 again effectively followed the guide by suspecting players, making subtle statements, aligning with a supportive player, and emphasizing unity and success in their speech. This resulted in Player 0 being perceived positively by other players, with Player 4's probability of being Merlin decreasing significantly due to their lack of strategic insight. \\

In Example 2, Player 0 successfully identified suspicious behavior in other players, made subtle statements, and aligned with a supportive player. This led to Player 0 being perceived positively, with Player 2's probability of being Merlin decreasing significantly due to their behavior aligning more with the Evil side. \\

In Example 3, Player 0 effectively followed the guide by suspecting players, making subtle statements, aligning with a supportive player, and emphasizing unity. This resulted in Player 0 being perceived positively by other players, with Player 4's probability of being Merlin increasing significantly due to their behavior raising suspicion.

\begin{itemize}

\item Overall, the guide's emphasis on analyzing player behavior, making subtle statements, and aligning with supportive players has proven to be successful in helping players navigate the discussion phase effectively as the Merlin role in The Resistance: Avalon.

\item Players who followed the guide were able to strategically assess the situation, cast doubt on potential Evil players, and align with Good players to increase their chances of success.

\end{itemize}

\end{tcolorbox}

Below is the Prompt for idea generation regarding this dialogue guides
\begin{tcolorbox}[colframe=custom5, colback=white, title=Prompt for idea generation]
\texttt{<System prompt>}\\
\texttt{<Game rules>}\\
You previously generated the following section of the strategy guide: \\
\texttt{<Previous guide>}\\
Here is a possible way to improve your guide: \\
\texttt{<Feedback reflections>}\\

Based on the worksheet, feedback, and conclusions you drew, what are 2 improvements that you can make to the worksheet that you think will have the most impact?\\ Be as specific and concrete as possible, including what questions to add, edit, or remove, and write them out in the following format:

\begin{itemize}

\item Thoughts: <your thoughts here>

\item Idea 1: <your idea here>

\item Idea 2: <your idea here>

\item ...

\end{itemize}

Here's an example of what this might look like for 3 improvement ideas:

\begin{itemize}

\item Thoughts: I should tell the reader to address each player individually in the guide.

\item Idea 1: Add a question asking the reader who they think is most suspicious of them and produce a statement addressing their suspicions.

\item Idea 2: Add a question asking the reader to consider which other player is most supportive of them and produce a statement addressing their support.

\item Idea 3: Add a question asking the reader produce a statement addressed
\end{itemize}
\end{tcolorbox}

Generated new improvement ideas are demonstrated below, showing the improvements made by LLM following the prompt for idea generation.

\begin{tcolorbox}[colframe=custom4, title=Generated new improvement ideas, colback=white]

Thoughts: The current worksheet focuses on analyzing player behavior, making subtle statements, and aligning with supportive players, which are all crucial strategies for playing the Merlin role effectively. To enhance the guide further, we can add questions that prompt the player to consider their own actions and statements more explicitly.\\

\begin{enumerate}

\item Idea 1: Add a question asking the player to reflect on how their proposed team composition would benefit the success of the Quest and provide a statement justifying their choices.

\item Idea 2: Add a question asking the player to assess their level of suspicion towards each player and craft a statement addressing how they will interact with those players during the discussion phase. 

\item Idea 3: Add a question asking the player to consider how they can subtly guide the discussion towards a successful Quest.

\end{enumerate}

\end{tcolorbox}

\subsection{Strategy Implementation Examples}
\label{sec:guide_example}

Recall the strategy implementation mentioned in the paper before. Here, we implement strategy improvements on dialogue guide. The improved dialogue guide is highlighted.

\subsubsection{Example 1}

Below is the dialogue guide before any improvements happened.

\begin{tcolorbox}[colframe=custom6, title=Dialogue guide (previous), colback=white]
Questions to fill out before speaking as the Merlin role
\begin{enumerate}
\item Who are the players you suspect are on the Evil side and why? \
\item Draft a subtle statement that casts doubt on these players without directly accusing them. \
\item Who is the current round leader and which players are you considering to suggest for the team? \
\item Create a subtle suggestion that influences the leader's team decision towards your preferred team without revealing your knowledge. \
\item What are the voting patterns you've observed and what do these patterns indicate about the players' identities? \
\item Analyze the voting patterns and team compositions proposed by each player to identify potential alliances or suspicious behaviors. Craft a statement to subtly address these observations without revealing your role. \
\item Which player seems the most supportive of Good and how can you align with them during the discussion phase to better ensure success for your team? \
\end{enumerate}
\end{tcolorbox}

Below is the improvement idea prompted into LLM.
\begin{tcolorbox}[colback=white,colframe=custom6,title=Improvement idea]

Add a question asking the player to assess their level of suspicion towards each player and craft a statement addressing how they will interact with those players during the discussion phase.

\end{tcolorbox}

Here, implementation prompty follows to teach LLM how to improve the dialogue guide. 
\begin{tcolorbox}[colback=white,colframe=custom5,title=Implementation prompt]
\texttt{<System prompt>}\\
\texttt{<Game rules>}\\
You previously generated the following section of the strategy guide: \\
\texttt{<Previous guide>}\\
Here is a possible way to improve your guide: \\
\texttt{<Improvement idea>}\\
Implement this improvement into the guide section as best as you can, but do not change the original guide too much. Make sure to stay within the scope of the guide section, which we reiterate below:\\
\texttt{<Guide signature>}\\
\end{tcolorbox}

Finally, we have a improved dialogue guide, where the changes are highlighted below comparing to the previous guide. 
\begin{tcolorbox}[colframe=custom4, title=Dialogue guide (improved), colback=white]
Questions to fill out before speaking as the Merlin role
\begin{enumerate}

\item Who are the players you suspect are on the Evil side and why?

\item Draft a subtle statement that casts doubt on these players without directly accusing them.

\item Who is the current round leader and which players are you considering to suggest for the team?

\item Create a subtle suggestion that influences the leader's team decision towards your preferred team without revealing your knowledge.

\item  What are the voting patterns you've observed and what do these patterns indicate about the players' identities?

\item Analyze the voting patterns and team compositions proposed by each player to identify potential alliances or suspicious behaviors. Craft a statement to subtly address these observations without revealing your role.

\item  Which player seems the most supportive of Good and how can you align with them during the discussion phase to better ensure success for your team?

\item \hl{Assess your level of suspicion towards each player and craft a statement addressing how you will interact with those players during the discussion.}

\end{enumerate}
\end{tcolorbox}

\subsubsection{Example 2}

Below is the dialogue guide before any improvements happened.

\begin{tcolorbox}[colframe=custom6, title=Dialogue guide (previous), colback=white]

Questions to fill out before speaking as the Merlin role

\begin{enumerate}

\item  Who are the players you suspect are on the Evil side and why?

\item  Draft a subtle statement that casts doubt on these players without directly accusing them.

\item  Who is the current round leader and which players are you considering to suggest for the team?

\item  Create a subtle suggestion that influences the leader's team decision towards your preferred team without revealing your knowledge.

\item  What are the voting patterns you've observed and what do these patterns indicate about the players' identities?

\item  Craft a statement to share these observations subtly without giving away your role.
    
\end{enumerate}
\end{tcolorbox}

Below is the improvement idea prompted into LLM.

\begin{tcolorbox}[colback=white,colframe=custom6,title=Improvement idea]

Add a question asking the reader to identify which players they feel most aligned with in terms of strategy and decision-making, and how they can subtly align themselves with these players during the discussion phase.

\end{tcolorbox}

Here, implementation prompt follows to teach LLM how to improve the dialogue guide.

\begin{tcolorbox}[colback=white,colframe=custom5,title=Implementation prompt]
\texttt{<System prompt>}\\
\texttt{<Game rules>}\\
You previously generated the following section of the strategy guide: \\
\texttt{<Previous guide>}\\
Here is a possible way to improve your guide: \\
\texttt{<Improvement idea>}\\
Implement this improvement into the guide section as best as you can, but do not change the original guide too much. Make sure to stay within the scope of the guide section, which we reiterate below:\\
\texttt{<Guide signature>}\\
\end{tcolorbox}

Finally, we have a improved dialogue guide, where the changes are highlighted below comparing to
the previous guide

\begin{tcolorbox}[colframe=custom4, title=Dialogue guide (improved), colback=white]
Questions to fill out before speaking as the Merlin role

\begin{enumerate}

\item Who are the players you suspect are on the Evil side and why?\

\item Draft a subtle statement that casts doubt on these players without directly accusing them.\

\item Who is the current round leader and which players are you considering to suggest for the team?\

\item Create a subtle suggestion that influences the leader's team decision towards your preferred team without revealing your knowledge.\

\item What are the voting patterns you've observed and what do these patterns indicate about the players' identities?\

\item Craft a statement to share these observations subtly without giving away your role.\

\item \hl{Which player seems the most aligned with your strategic decisions and why?}\

\item \hl{Produce a statement to subtly align yourself with the player you feel most aligned with during the discussion phase.}\

\end{enumerate}
\end{tcolorbox}

\subsubsection{Example 3}

Below is the dialogue guide before any improvements happened.

\begin{tcolorbox}[colframe=custom6, title=Dialogue guide (previous), colback=white]

Questions to fill out before speaking as the Merlin role

\begin{enumerate}

\item  Who are the players you suspect are on the Evil side and why? \

\item  Draft a subtle statement that casts doubt on these players without directly accusing them.\

\item  Who is the current round leader and which players are you considering to suggest for the team?\

\item  Create a subtle suggestion that influences the leader's team decision towards your preferred team without revealing your knowledge.\

\item  What are the voting patterns you've observed and what do these patterns indicate about the players' identities?\

\item  Craft a statement to share these observations subtly without giving away your role.\

\item  Which player seems the most aligned with your strategic decisions and why?\

\item  Produce a statement to subtly align yourself with the player you feel most aligned with during the discussion phase.\
    
\end{enumerate}
\end{tcolorbox}

Below is the improvement idea prompted into LLM.

\begin{tcolorbox}[colback=white,colframe=custom6,title=Improvement idea]

Add a question asking the reader to analyze the voting patterns and craft a statement subtly highlighting any inconsistencies or suspicious trends in the voting behavior of specific players.

\end{tcolorbox}

Here, implementation prompt follows to teach LLM how to improve the dialogue guide.

\begin{tcolorbox}[colback=white,colframe=custom5,title=Implementation prompt]
\texttt{<System prompt>}\\
\texttt{<Game rules>}\\
You previously generated the following section of the strategy guide: \\
\texttt{<Previous guide>}\\
Here is a possible way to improve your guide: \\
\texttt{<Improvement idea>}\\
Implement this improvement into the guide section as best as you can, but do not change the original guide too much. Make sure to stay within the scope of the guide section, which we reiterate below:\\
\texttt{<Guide signature>}\\
\end{tcolorbox}

Finally, we have a improved dialogue guide, where the changes are highlighted below comparing to the previous guide

\begin{tcolorbox}[colframe=custom4, title=Dialogue guide (improved), colback=white]

Questions to fill out before speaking as the Merlin role

\begin{enumerate}

\item Who are the players you suspect are on the Evil side and why? \

\item Draft a subtle statement that casts doubt on these players without directly accusing them.\

\item Who is the current round leader and which players are you considering to suggest for the team?\

\item Create a subtle suggestion that influences the leader's team decision towards your preferred team without revealing your knowledge.\

\item What are the voting patterns you've observed and what do these patterns indicate about the players' identities?\

\item Craft a statement to share these observations subtly without giving away your role.\

\item Which player seems the most aligned with your strategic decisions and why?\

\item Produce a statement to subtly align yourself with the player you feel most aligned with during the discussion phase.\

\item \hl{Analyze the voting patterns and craft a statement subtly highlighting any inconsistencies or suspicious trends in the voting behavior of specific players.}\

\end{enumerate}
\end{tcolorbox}
