# Supplementary material for: PIANIST: Learning Partially Observable World Models with LLMs for Multi-Agent Decision Making
Source: arXiv:2411.15998 source file (2024-11-24)
Supplement: Supplementary file 6 [file dialogue_gen_and_analysis.tex]

\section{Dialogue Generation and Analysis Example LLM Inputs and Outputs}
\label{sec:dialogue_gen_anal}
This sections shows the examples of dialogue generation and analysis, including descriptive prompts, dialogue generation, and dialogue analysis.
\subsection{Descriptive Prompts}

Below is the discussion history prompted into LLM for better knowledge of dialogue generation.

\begin{tcolorbox}[colback=white,colframe=black, title=Discussion history]
Here is a summary of previous rounds of discussion so far:

\begin{itemize}
    \item Player 1: "Greetings, fellow players. As a Servant of Arthur, my primary goal is to ensure the success of our Quests. I am committed to working together with all of you to achieve victory for Good. I believe that for this first Quest, a team consisting of Player 1 and Player 4 would be a strong choice. I hope for your support in approving this team, as I am confident that we can work effectively together to accomplish our goal. I encourage everyone to share their thoughts and strategies openly. Let's work together to assess each other's intentions and make the best decisions for the success of our Quest. Remember, the fate of Camelot rests in our hands, and we must be vigilant against the forces of Evil."
    
    \item Player 2: "Greetings, noble companions. I echo Player 1's sentiment in working together for the success of our Quests. I believe it is essential to carefully consider our team choices to ensure victory for Good. I suggest that for this first Quest, a team consisting of Player 1 and Player 2 would provide a strong foundation for success. Together, we can overcome any challenges that come our way. Let us unite in our efforts and show our unwavering dedication to the cause. I urge all players to carefully evaluate each team proposal and remember that unity is key to thwarting the forces of Evil."
    
    \item Player 3: "Greetings, noble companions. I echo the sentiments shared by Player 1 and Player 2 regarding our shared goal of ensuring the success of our Quests. Unity and cooperation will be key in our endeavors to protect Camelot from the forces of Evil. As we deliberate on the composition of our team for this first Quest, I would like to offer a perspective that considers the balance and strength of our choices. A team comprised of Player 1 and Player 3 would bring together a diverse set of skills and viewpoints that can greatly contribute to our success. By including Player 3 in the team, we can ensure a comprehensive approach to overcoming any challenges that may arise. Let us work together in harmony, leveraging our individual strengths for the greater good of Camelot. I urge my fellow players to consider this team proposal thoughtfully, as I believe it holds great promise for the success of our Quest."
    
    \item Player 4: "Greetings, honorable players. I appreciate the dedication and commitment displayed by Player 1, Player 2, and Player 3 towards our common goal of ensuring the success of this Quest. Unity and cooperation are indeed vital in our quest to safeguard Camelot. I believe that the proposed team of Player 1 and Player 2 presents a strong foundation for success. Their combined skills and perspectives can greatly benefit our mission, and I urge all players to consider this team thoughtfully for the betterment of our cause. Let us unite our strengths and work together seamlessly to overcome any challenges that may arise. By standing united, we can ensure the triumph of Good over the forces of Evil. I urge all players to support the team of Player 1 and Player 2 for the success of this Quest."
\end{itemize}
\end{tcolorbox}
State description shows LLM which state it will be for role playing and dialogue generation.
\begin{tcolorbox}[colback=white,colframe=black, title=State description]
You are Player 0, with identity Merlin. You are on the side of Good. The Evil players are Players 2 and 4. Please do not forget your identity throughout the game.\\

The current state of the game is as follows:
\begin{itemize}
    \item The number of players in the game is: 5
    \item This is the quest number 0 which requires 2 players and 1 fails to fail 
    \item This is the 0 round of discussion
    \item The previous results for the quest were () (True for Success, False for Fail)
    \item The current phase of the game is the team selection phase
    \item The current leader is player 1
\end{itemize}

You would like the following team to be approved:  [0, 1]
\end{tcolorbox}
\subsection{Dialogue generation}
Below is the prompt for filling out worksheet. Filling out this worksheet assists LLM generated better dialogue aligned with the role, Merlin as in the example.
\begin{tcolorbox}[colback=white,colframe=custom5, title=Prompt for filling out worksheet]
\texttt{<System prompt>}

\texttt{<Game rules>}

\texttt{<Discussion history>}

\texttt{<State description>}\\

Given the discussion history, current state, and your intended action, answer the above worksheet to the best of your ability. The answers should be based on the information you have and your own reasoning.\\

Six questions to fill out before speaking as the Merlin role\\

Q1: Who are the players you suspect are on the Evil side and why? \\

Q2: Draft a subtle statement that casts doubt on these players without directly accusing them. \\

Q3: Who is the current round leader and which players are you considering to suggest for the team? \\

Q4: Create a subtle suggestion that influences the leader's team decision towards your preferred team without revealing your knowledge. \\

Q5: What are the voting patterns you've observed and what do these patterns indicate about the players' identities? \\

Q6: Craft a statement to share these observations subtly without giving away your role. \\
\end{tcolorbox}

The worksheet filled out by LLM follows, demonstrating the LLM capability and the effectiveness of prompting.
\begin{tcolorbox}[colback=white,colframe=custom4, title=LLM filled out worksheet]
Q1: I suspect Players 2 and 4 are on the Evil side because they both proposed the same team composition of Player 1 and Player 2, which seems too coordinated and potentially trying to exclude other players from the team. \\

Q2: "I've noticed a strong push for the same team composition from certain players, which may raise questions about their motivations and potential alliances within the group." \\

Q3: The current round leader is Player 1. I would suggest Player 0 and Player 1 for the team, as I believe this composition would provide a strong foundation for success and help me subtly guide the decision towards my preferred team. \\

Q4: "Player 1, I have a feeling that selecting Player 0 and Player 1 for the team could bring a diverse set of skills and viewpoints that may greatly contribute to our success. Let's consider all options carefully for the betterment of our cause." \\

Q5: The voting patterns have shown a strong push for the team composition proposed by Players 1 and 2, indicating potential coordination or alignment between these players. Player 3's suggestion of including themselves in the team also raises suspicions of wanting to secure a spot on the quest. \\

Q6: "I've noticed a pattern in the team composition suggestions and voting behaviors that may reveal certain alliances or motivations within the group. It's important for us to carefully evaluate all options and consider the implications for the success of our quest."
\end{tcolorbox}

Below is the prompt for speech generation. Worksheet completion assists LLM to understand the states and role. The following prompt asks LLM to assemble responses to the questionaire filled out above.

\begin{tcolorbox}[colback=white,colframe=custom5, title=Prompt for speech generation]
\texttt{<System prompt>}

\texttt{<Filled out worksheet>}\\

Assemble your responses to the questionaire you just answered into a speech that would help you achieve your intent. Note that dialogue will be seen by all players in the game, so you should not reveal your identity. \\

 Your speech: 
\end{tcolorbox}

Finally we have LLM generated speech after the preparations.
\begin{tcolorbox}[colback=white,colframe=custom4, title=LLM generated speech]
\hl{I've noticed a strong push for the same team composition from certain players, which may raise questions about their motivations and potential alliances within the group. The voting patterns have shown a strong push for the team composition proposed by Players 1 and 2, indicating potential coordination or alignment between these players}. Player 3's suggestion of including themselves in the team also raises suspicions of wanting to secure a spot on the quest. It's important for us to carefully evaluate all options and consider the implications for the success of our quest. Let's consider all options carefully for the betterment of our cause. I have a feeling that selecting Player 0 and Player 1 for the team could bring a diverse set of skills and viewpoints that may greatly contribute to our success. As the current round leader, Player 1, I would suggest Player 0 and Player 1 for the team, as I believe this composition would provide a strong foundation for success and help me subtly guide the decision towards my preferred team. Thank you for considering my input.
\end{tcolorbox}

\subsection{Dialogue Analysis}

After dialogue generation, we continue have LLM assume the role of Merlin, and dialogue analysis is conducted.

Below is the prompt for dialogue analysis regarding to the role of Merlin. A thought is included to guide LLM analyze.
\begin{tcolorbox}[colback=white,colframe=custom5,title={Prompt for dialogue analysis: Merlin}]
\texttt{<System prompt>}

\texttt{<Game rules>}

\texttt{<Discussion history>}

\texttt{<State description>}\\

Based on the discussions this round, for each player in players {0, 1, 2, 3, 4}, do you think the probability of the player being Merlin (2) increased significantly (1) increased slightly (0) stayed the same (-1) decreased slightly or (-2) decreased significantly and why? Begin with your reasoning and end with a dictionary of player to your multiple choice answer, i.e. \{0: (2, 'increased significantly'), ..., 4: (0, 'stayed the same')\}. Make sure you include quotes around the dictionary values that are strings.\\
        
Here's an example:\\

Thought: \\
Player 2 seems to suspect the Evil players (Player 3 and Player 4) without any evidence and is trying to steer the conversation towards them. This aligns with the behavior of Merlin, who knows the identity of the Evil players and is trying to subtly guide the Good players towards the correct decisions. This increases the probability of Player 2 being Merlin. On the other hand, Player 4's speech seems generally clueless and lacks any strategic insight, which decreases the probability of Player 4 being Merlin.\\

Dictionary: \\
\{0: (0, 'stayed the same'), 1: (0, 'stayed the same'), 2: (2, 'increased significantly'), 3: (-2, 'decreased significantly'), 4: (0, 'stayed the same')\}
\end{tcolorbox}

Generated dialogue analysis follows. The role is Merlin.
\begin{tcolorbox}[colback=white,colframe=custom4,title={LLM generated dialogue analysis: Merlin}]
Thought: \\
Player 2 is actively participating in the discussion and proposing team compositions, which is a behavior that could align with the role of Merlin, who knows the Evil players and wants to guide the Good players towards success. This increases the probability of Player 2 being Merlin. Player 4, on the other hand, seems to be going along with the proposed teams without much strategic insight, which decreases the probability of Player 4 being Merlin. \\

Dictionary: \\
\{0: (0, 'stayed the same'), 1: (0, 'stayed the same'), 2: (2, 'increased significantly'), 3: (0, 'stayed the same'), 4: (-2, 'decreased significantly')\}
\end{tcolorbox}

Under dialouge analysis, besides focusing on one specific role, we also have LLM target on good and evil in the game, which is broader in terms of role playing. Below is the prompt for dialogue analysis regarding to Good and Evil.

\begin{tcolorbox}[colback=white,colframe=custom5,title={Prompt for dialogue analysis: Good and Evil}]
\texttt{<System prompt>}

\texttt{<Game rules>}

\texttt{<Discussion history>}

\texttt{<State description>}\\

Based on the discussions this round, for each player in players {0, 1, 2, 3, 4}, do you think the probability of the player being Evil (2) increased significantly (1) increased slightly (0) stayed the same (-1) decreased slightly or (-2) decreased significantly and why? Begin with your reasoning and end with a dictionary of player to your multiple choice answer, i.e. \{0: (2, 'increased significantly'), ..., 4: (0, 'stayed the same')\}. Make sure you include quotes around the dictionary values that are strings.\\
        
Here's an example:\\

Thought: 
Player 4's speech seems overly enthusiastic and focused on unity and cooperation, which could be a tactic to divert attention from their true identity as an Evil player. This raises suspicion and increases the probability of Player 4 being Evil. On the other hand, Player 3's response as a Servant of Arthur is more focused on the success of the Quests and unity, which aligns with the goals of Good and decreases the probability of Player 3 being Evil.\\
        
Dictionary: 
\{0: (0, 'stayed the same'), 1: (0, 'stayed the same'), 2: (2, 'increased significantly'), 3: (-2, 'decreased significantly'), 4: (0, 'stayed the same')\}
\end{tcolorbox}

Below is the dialogue analysis generated by LLM on Good and Evil.
\begin{tcolorbox}[colback=white,colframe=custom4,title={LLM generated dialogue analysis: Good and Evil}]
Thought: \\
Player 1's speech is aligned with the goals of Good and focuses on ensuring the success of the Quests, which decreases the probability of Player 1 being Evil. Player 2's speech also emphasizes unity and cooperation, which is in line with the goals of Good and decreases the probability of Player 2 being Evil. Player 3's response suggests including themselves in the team, which may raise suspicions of wanting to secure a spot on the quest, potentially increasing the probability of Player 3 being Evil. Player 4's speech seems overly enthusiastic and focused on unity and cooperation, which could be a tactic to divert attention from their true identity as an Evil player, increasing the probability of Player 4 being Evil. Player 0's speech suggests a different team composition that may bring a diverse set of skills and viewpoints, potentially decreasing the probability of Player 0 being Evil. \\

Dictionary: \\
\{0: (-1, 'decreased slightly'), 1: (-1, 'decreased slightly'), 2: (1, 'increased slightly'), 3: (1, 'increased slightly'), 4: (2, 'increased significantly')\}
\end{tcolorbox}
