# Supplementary material for: PIANIST: Learning Partially Observable World Models with LLMs for Multi-Agent Decision Making
Source: arXiv:2411.15998 source file (2024-11-24)
Supplement: Supplementary file 7 [file dialogue_guide_improve.tex]

\section{Dialogue Guide Improvement Evaluation Implementation Details}
\label{sec:dialogue_guide_improve}

We provide more details on our dialogue improvement evaluation process here and as shown in figure \ref{fig:dialogueimprove}. The improvement method (skill coach) remains the same as we described before. 

We first generate a synthetic dataset by simulating a game of Avalon with initial dialogue and move policies $\boldsymbol{\phi}$. Given the dialogue guide $\sigma$ we want to evaluate, we then sample `scenarios' from the dataset. A scenario consists of a game state, intended action, and private information in the simulated trajectory. We create an Avalon agent like the one we described in \ref{sec:avalon_agent} for each player in the game, initialized with their corresponding private information. The Avalon agent is then asked to generate dialogue using the dialogue guide $\sigma$. 

Using this new generated dialogue, we then simulate the next round of dialogue analysis for each Avalon agent. This produces analysis scores based on how likely they think the player is to be Merlin $z_{merlin}$, and how likely they think the player is to be Evil $z_{evil}$, where $z_{merlin}, z_{evil} \in [-2, 2]$. For evaluating Merlin, we get the average $z_{merlin}$ scores from the Evil players, $\bar{z}_{merlin}$, along with the average $z_{evil}$ scores from the Good players $\bar{z}_{evil}$. We then take the minimum of these two as the feedback score $z = \min \{\bar{z}_{evil}, \bar{z}_{merlin}\}$. This is because Merlin wants to both minimize the probability of being detected by the Evil players, and also minimize the probability of being identified as Evil by the Good players.

\begin{figure}[h]
    \centering
    \includegraphics[width = 1.0\textwidth]{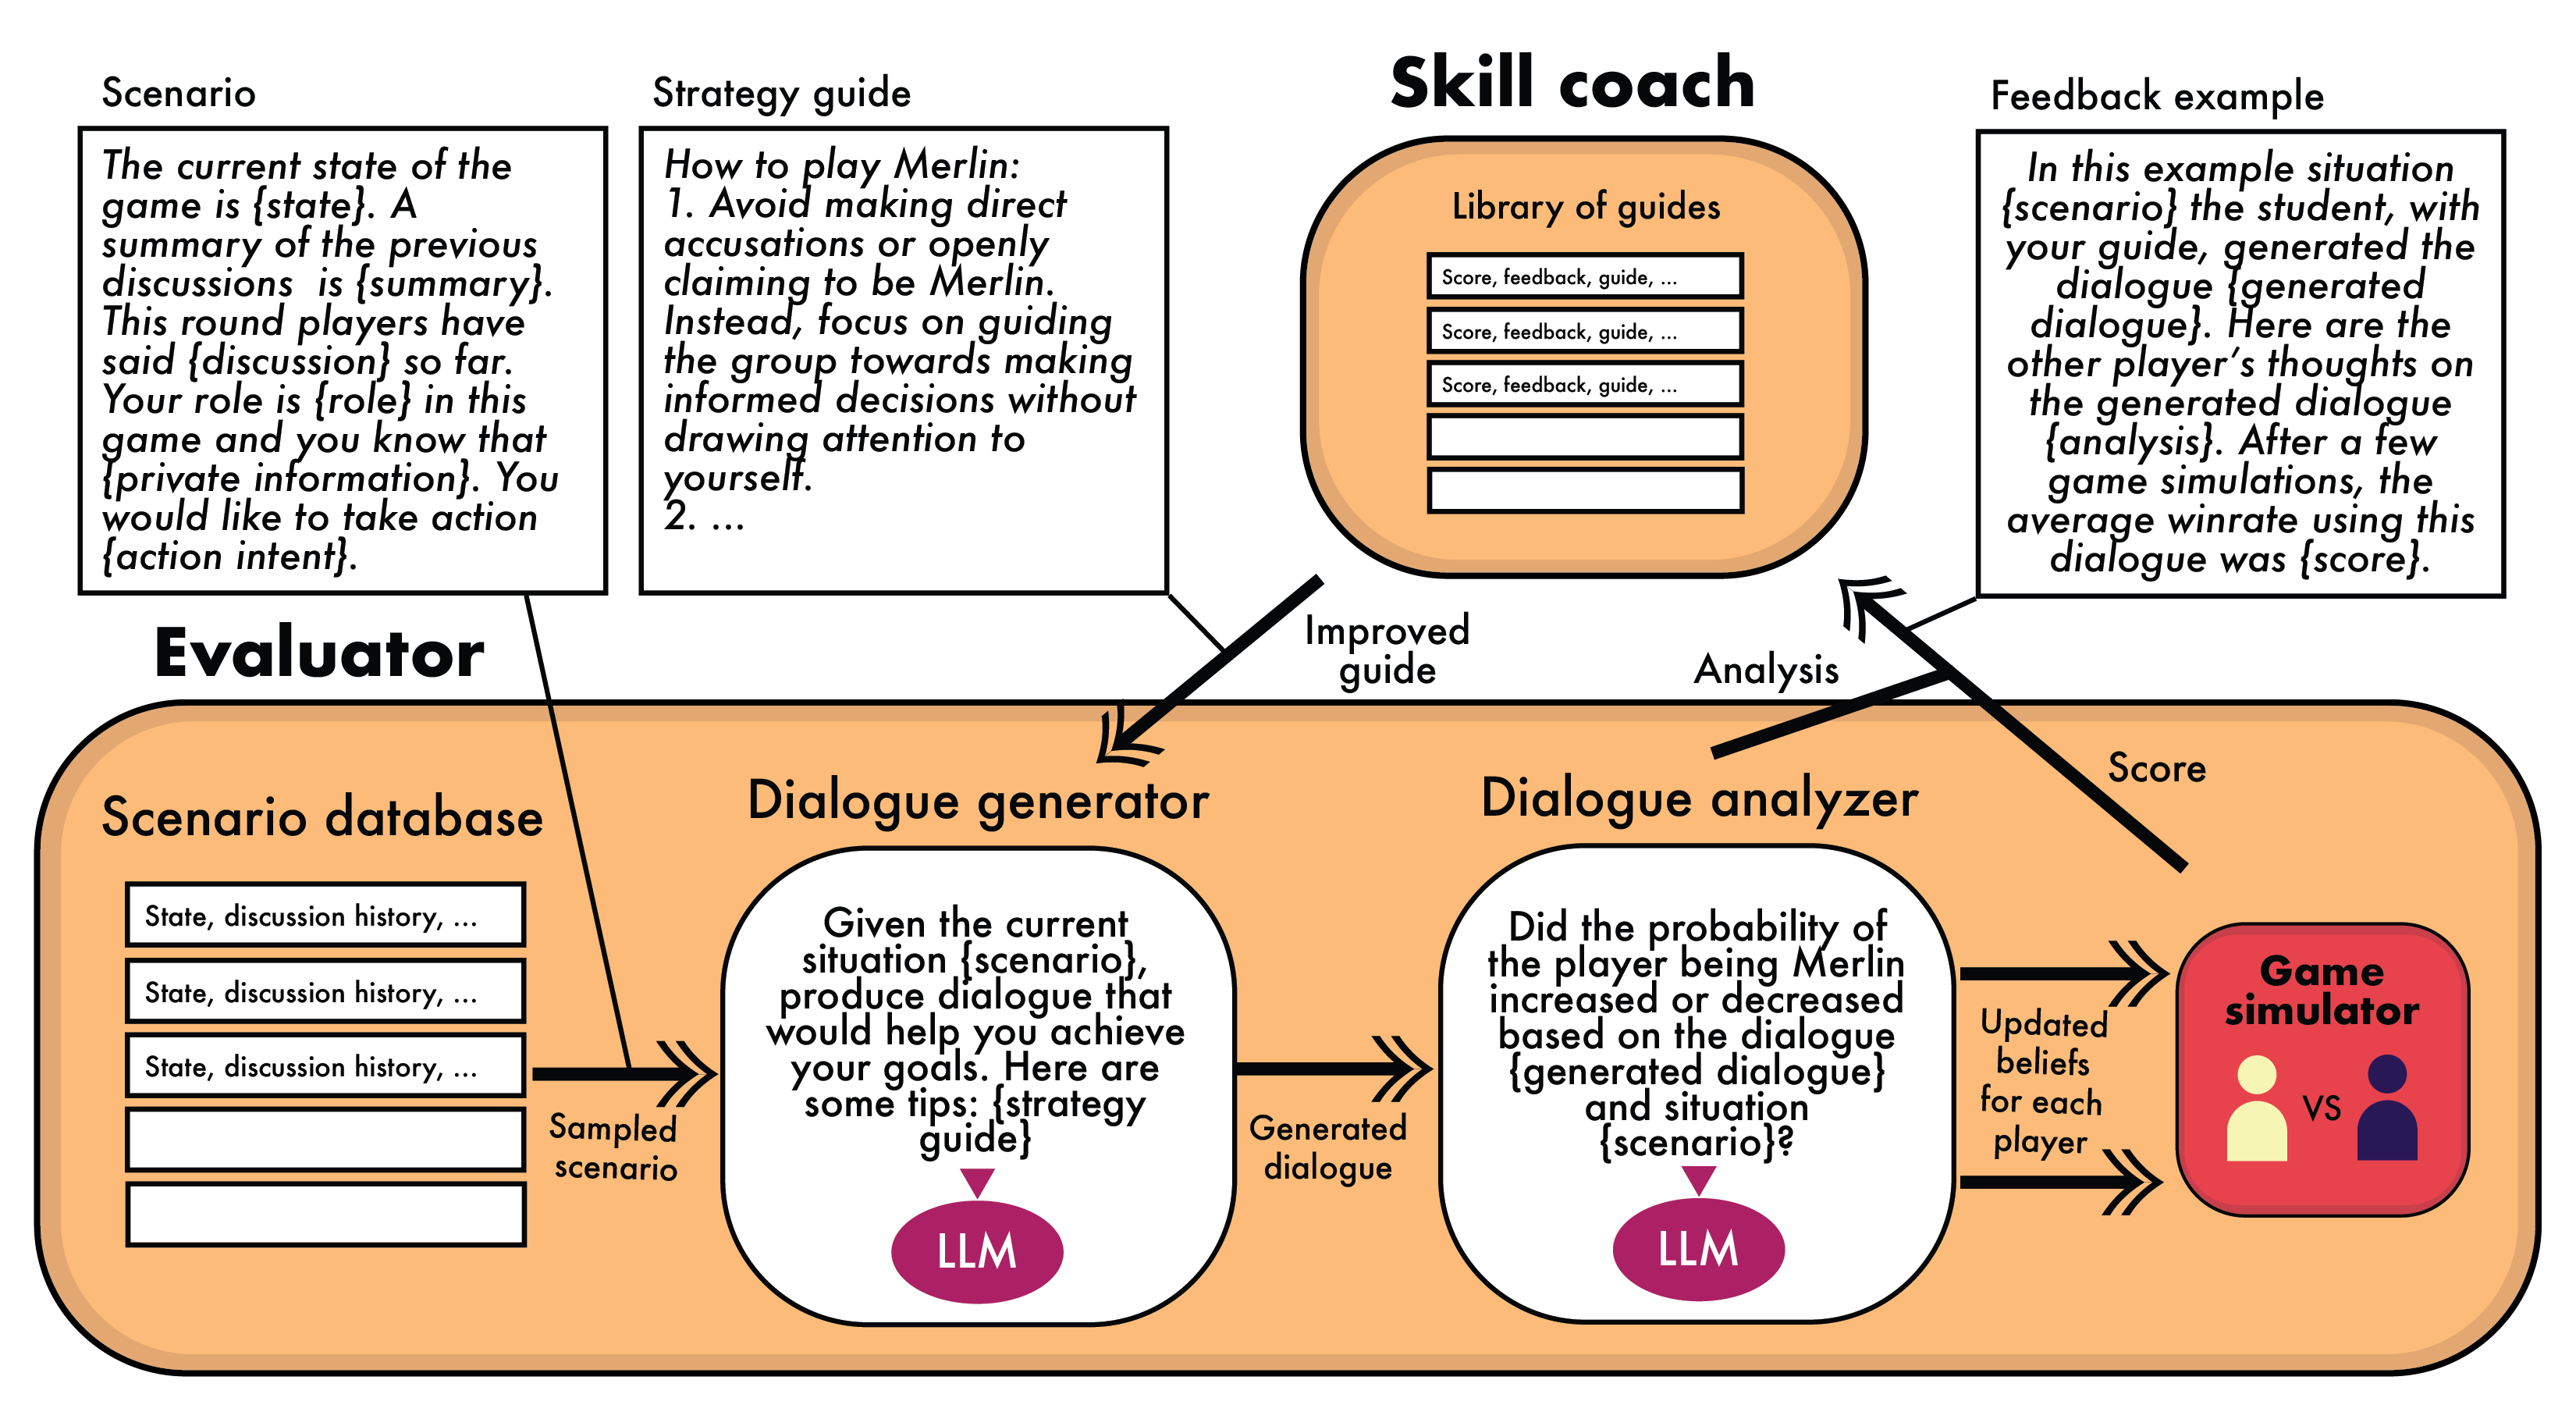}
    \caption{\textbf{Overview of our improvement process for learning dialogue generation strategies}. This includes how we evaluate the dialogue and how we collect feedback. The skill coach here can be implemented as either our improvement method, \method, or any of the baseline methods we described.}
    \label{fig:dialogueimprove}
\end{figure}

The dialogue analyzer (discriminator) is described in more detail in Appendix \ref{sec:avalon_agent} and the specific generation and analysis prompts are shown in Appendix \ref{sec:dialogue_gen_anal}.
