# Supplementary material for: PIANIST: Learning Partially Observable World Models with LLMs for Multi-Agent Decision Making
Source: arXiv:2411.15998 source file (2024-11-24)
Supplement: Supplementary file 8 [file improvement_details.tex]

\section{Improvement Process Implementation Details}

\begin{algorithm}[h!]
  \small
  \caption{\method Pseudocode}
  \label{alg:skillcoach}
  \SetKwInOut{Input}{Data}
  \Input{
    $T$: strategy tree storing strategy $s$, feedback ($\tau_s$), and priority score ($z_s$), 
    $Q$: idea queue, 
    `seed functions', 
    $N_{ideas}$: number of ideas, 
    $N_{strategies}$: number of strategies, 
    $N_{evolutions}$: number of evolutions,
    $N_{feedback\_examples}$: number of states of give as feedback,
  }
  
  \SetKwFunction{GenerateIdeas}{generate\_ideas}
  \SetKwFunction{ImplementStrategies}{implement\_strategies}
  \SetKwFunction{SelectStrategy}{select\_strategy}
  \SetKwFunction{SelectIdea}{select\_idea}
  \SetKwFunction{SelectKeyStates}{select\_key\_states}
  \SetKwProg{Fn}{Function}{:}{}

  \Fn{\SelectStrategy{$T$}}{
    $\sigma_{\text{best}} \gets \underset{\sigma \in T_2}{\arg}\text{softmax} z_\sigma$ \tcp{one possible implementation where you take one of the best two strategies in the whole tree randomly (BFS2)}
    \Return{$s_{\text{best}}$}
  }

  \Fn{\SelectIdea{$Q, \sigma$}}{
    $d_{\text{best}} \gets \operatorname{softargmax}_{d \in Q} UCB(z_d, n_d)$ \tcp{one possible implementation where you take the best strategy in the queue using softmax UCB, $z_d$ being the empirical $q$-value and $n_d$ being the number of tries}
    \Return{$\sigma_{\text{best}}$}
  }

  \Fn{\SelectKeyStates{$\tau_\sigma$}}{
     $K_\sigma \gets \underset{s \in \tau}{\text{arg}}\max_k (\operatorname{SearchEstimate}(s) - v_{\sigma}(s))^2$ \tcp{one possible way to select key states for $\sigma$ that is a value heuristic $v_\sigma$}
     \Return{$K_\sigma$}
  }
  
  \Fn{\GenerateIdeas{$N_{ideas}$}}{
    % \For{$i \gets 1$ \KwTo $N_{ideas}$}{
    $\sigma \gets$ \SelectStrategy{$T$}\;
    $K_\sigma \gets$ \SelectKeyStates($\tau_\sigma$) \tcp{$K_\sigma$ is a set of key states from the trajectory feedback $\tau_\sigma$ for strategy $\sigma$}
    % \tcp{$K_s$ is the set of key states in the simulated feedback trajectory}
    % $\text{Str}_{\text{natural language feedback}} \gets$ TranslateToNaturalLanguage($K_s$)\;
    $D_{\text{new ideas}} \gets$ LLM(Generate $N_{ideas}$ new ideas based on string description of $K_\sigma$, which includes the output of the strategy, action taken, state description, final outcome of the trajectory, search estimate of the state, and any intermediate values used to compute the output of the strategy)\;
    \For{$d \in D_{\text{new ideas}}$}{
        Store $d$ in $Q$ with prior score $z_{d} = 0.0$ and $n_d = 0$\;
    }
    % }
  }
  
  \Fn{\ImplementStrategies{$N_{strategies}$}}{
    
    $\Sigma_{\text{new}}, D, P = \texttt{[]}, \texttt{\{\}}, \texttt{\{\}}$ \tcp{list of new generated strategies, dictionary mapping new generated strategy to the idea that generated it, and dictionary mapping generated strategies to their parents}
    \For{$i \gets 1$ \KwTo $N_{strategies}$}{
    $\sigma \gets$ \SelectStrategy{$T$}\;
        % $\sigma, d \gets$ SelectStrategyAndIdea($T$, $Q$, $N_{strategies}$) using the exploratory tree selection policy based on priority scores ($z_\sigma, z_d$)\;
        $d \gets$ \SelectIdea{$Q, \sigma$}\;
        $\sigma_{\text{new}} \gets$ LLM(Improve $\sigma$ using $d$)\;
        $\Sigma_{\text{new}}.\text{append}(\sigma_{\text{new}})$\;
        $D[\sigma_{\text{new}}] = d$\;
        $P[\sigma_{\text{new}}] = \sigma$\;
    }
    $W, \mathcal{T} \gets$ SelfplaySimulate($\Sigma_{\text{new}} \cup \operatorname{unique}(P.\text{values})$) \tcp{simulate games, getting average winrates $W[\sigma]$ for each strategy $\sigma$ and simulated trajectory feedback $\mathcal{T}[\sigma]$}
    \For{$\sigma \in \Sigma_{\text{new}}$}{
        $T.\text{add}(\sigma, P[\sigma], D[\sigma])$ \tcp{add new strategy to tree from parent based on idea}
        $z_{\sigma} \gets W[\sigma]$ \tcp{add function score}
        $z_{D[\sigma]} \gets \frac{n_{D[\sigma]}}{n_{D[\sigma]}+1}z_{D[\sigma]} + \frac{1}{n_{D[\sigma]}+1}(W[\sigma] - W[P[\sigma]])$ \tcp{update idea score with how much it improved the strategy by}
    }
  }
  
  \Repeat{$N_{\text{evolutions}}$}{
    \GenerateIdeas{$N_{\text{ideas}}$}\;
    \ImplementStrategies{$N_{\text{strategies}}$}\;
  }
  
  \Return{Best strategies in $T$ according to their scores $z_s$}
\label{alg:method_pseudocode}
\end{algorithm}
