# Supplementary material for: PIANIST: Learning Partially Observable World Models with LLMs for Multi-Agent Decision Making
Source: arXiv:2411.15998 source file (2024-11-24)
Supplement: Supplementary file 9 [file improvement_methods.tex]

\section{Improvement method implementation details}

\begin{tcolorbox}[title=Thought prompt for Thought BFS]
Given the rules of the game, write down your thoughts and pseudocode for how to create a function to evaluate the value of a state in the game.\\
-----\\
Thoughts:\\
\textless your thoughts here. try to think about characteristics of the game that can help you\textgreater \\
-----\\
Pseudocode: \\
\textless the pseudocode for your function here. You can be as abstract as you want\textgreater \\
-----\\

Below is an example for the game of GOPS (Goofspiel), where I calculate the expected score for each player at the end of the game.
                               
\textquotedbl
Thoughts:
In GOPS, the value of a state can be determined by the current total score of each player, the remaining score cards in the deck, and the cards left in each player's hand.\\
- Winning a round with a high score card can significantly impact the total score, so having high-value cards left in hand is important.\\
- The distribution of score cards in the deck can also affect the value of a state, as certain cards may be more valuable than others.\\

Pseudocode:\\
1. Define a function evaluate\_state(state) that takes the current state of the game as input.\\
2. Calculate the total score of each player based on the current state.\\
3. Determine the remaining score cards in the deck and the cards left in each player's hand.\\
4. Evaluate the potential value of the state by considering factors such as:\\
   - The difference in total scores between the players\\
   - The value of the cards left in each player's hand\\
   - The distribution of score cards in the deck\\
5. Return a tuple containing the expected score for the current player and the opponent player at the end of the game.\\
\end{tcolorbox}
