# Supplementary material for: PIANIST: Learning Partially Observable World Models with LLMs for Multi-Agent Decision Making
Source: arXiv:2411.15998 source file (2024-11-24)
Supplement: Supplementary file 10 [file rl_implementation.tex]

\section{Details on Learning the Value Heuristic via Reinforcement Learning}
\label{sec:rl_implementation}

% {\color{blue}{

% Then our \textbf{goal is to find the optimal strategy} $\sigma_i$ that approximates finding the optimal policy, i.e. 
% % \[\argmax\limits_{\sigma_i}{\mathbb{E}}\limits_{\tau \sim (f(\sigma_i), \phi_{-i})}\]

% \[\argmax_{\sigma_i}\underset{\phi_{-i} \sim \pi_{\phi_{-i}}, \tau \sim (f(\sigma_i), \phi_{-i})}{\mathbb{E}} \left[ \sum_{(s,a) \in \tau} R_i(s,a) \right] \approx \argmax_{\phi_i}\underset{\phi_{-i} \sim \pi_{\phi_{-i}}, \tau \sim (\phi_i, \phi_{-i})}{\mathbb{E}} \left[ \sum_{(s,a) \in \tau} R_i(s,a) \right]\]
% where $\tau$ is the simulated trajectory according to the joint policy. 

% }}

We employ Monte-Carlo based RL approach (\cite{sutton2018reinforcement}) to train a value heuristic for both five-player Avalon and five-card GOPS games. To do so, we construct a MSE loss in each episode for training the value function, i.e.,
\begin{align*}
    \argmin_\theta \sum_{i}^{\mathcal{N}} \sum_{t=0}^{T} \left(V_\theta^i(s_t)- Score^i (s_t) \right)^2
\end{align*}
where $\mathcal{N}$ represents the number of actors, $V_\theta^i(s_t), i=1, 2, \cdots, \mathcal{N}$ denotes the value function for each actor, and $T$ is the time horizon. Notice that $s_t$ and $Score^i (s_t)$ denote the state at time step $t$ and the corresponding cumulative reward for each actor, i.e., $\sum_{t}^T R_i (s_t, a_t)$. It is worth pointing that $Score^i (s_t)$ (the cumulative reward starting from $s_t$) is the unbiased estimate of the value function $V_\theta^i(s_t)$.

For both Avalon and GOPS games, the value function $V_\theta^i(s_t)$ is predicted by a neural network. We then train the value function network by minimizing the aforementioned loss function over episodes. In Avalon, we consider 20 evolutions (epochs) for the training process. At the end of each evolution, 30 batch runs (episodes) are generated and used to train the value function network, i.e., a total of 600 episodes for training. In GOPS, we train by 20 evolutions as well while considering 60 batch runs each (1200 episodes in total). We evaluate the final performance over 10 episodes in both games. The neural network is constructed by a multilayer perceptron (MLP) with 2 hidden layers. We select a hidden layer size of $128 * 128$ for Avalon and that of $64 * 64$ for GOPS. Likewise, the chosen learning rates are $5e-4$ and $8e-4$, respectively. The value function is expected to predict the score for each player in the game, e.g., two for GOPS and number of players for Avalon. All experimental hyper-parameters are summarized in Table~\ref{tab_rl_improve_parameter}.

Having introduced the set up, one can observe in Figure~\ref{fig_avalon_gops_rl_improve} an increased performance of RL-trained value heuristic in both five-player Avalon and five-card GOPS games. This validates the improvement for training value heuristic via reinforcement learning within limited evolutions.

\begin{figure}
\centering 
\subfigure[Avalon]
{
\begin{minipage}{0.48\linewidth}
\centering    
\includegraphics[width=\textwidth]{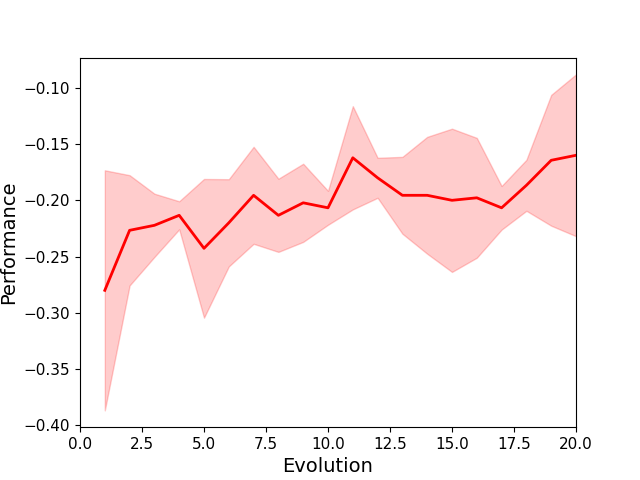} 
\end{minipage}
}
\subfigure[GOPS]
{
	\begin{minipage}{0.48\linewidth}
	\centering 
	\includegraphics[width=\textwidth]{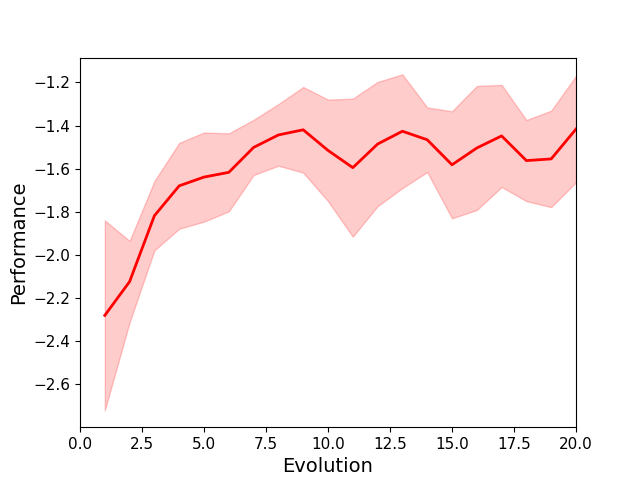} 
	\end{minipage}
}
\caption{The training curves of the value heuristic via reinforcement learning in five-player Avalon and five-card GOPS, averaged across five independent runs. The solid lines show the mean and the shaded areas depict the standard deviation.}
\label{fig_avalon_gops_rl_improve}
\end{figure}

\begin{table}[tp]
	\centering
	\fontsize{10}{10}\selectfont
	\begin{threeparttable}
		\caption{Summary of experimental hyper-parameters in RL-training value heuristic}
		\label{tab_rl_improve_parameter}
		\begin{tabular}{cccc}
        \hline
        \hline
			 Parameters & Avalon
			& GOPS  \cr
        \hline
            Type of neural network & MLP & MLP  \cr
            
            Number of hidden layers & 2 & 2  \cr

            Hidden layer size &  128*128 & 64*64   \cr

            Learning rate & 5e-4 & 8e-4  \cr

            Output dimension &  \# of players & 2  \cr

            Number of evolutions &  20 & 20   \cr
            
            Number of batch runs &  30 & 60   \cr

            Number of final batch runs &  10 & 10   \cr
        \hline
        \hline
		\end{tabular}
	\end{threeparttable}
\end{table}
