# Supplementary material for: PIANIST: Learning Partially Observable World Models with LLMs for Multi-Agent Decision Making
Source: arXiv:2411.15998 source file (2024-11-24)
Supplement: Supplementary file 11 [file vh_examples.tex]

\section{Value Heuristic LLM Prompt and Output Examples}

\subsection{System Prompts}

System prompt are guidelines for LLM to generate outputs align with the intended goals. In our case, the goal is to generate a function that evaluates the value of a state in a game under low cost.
\begin{tcolorbox}[title=Value heuristic system prompt,  colframe=custom3, colback=white]
You are a function engineer trying to write a function that can evaluate the value of a state in a game. This is known as a value heuristic, and will be used in look-ahead search algorithms to evaluate the value of unexplored states. Your goal is to develop a heuristic that is as accurate as possible without being too expensive to compute. Hence, you are not allowed to runs simulations in the function.\\
\end{tcolorbox}

The following example is a detailed prompt telling the LLM how to format the value heuristics specifically in the GOPS game. The format of input and output are clearly defined in the prompt with illustrations, examples and structures.

\begin{tcolorbox}[colback=white, colframe=black, title=GOPS value heuristics function signature]
The function (written in python) should be named `evaluate state' and take in a tuple called `state' of the game state as input. 
Specifically, the input tuple will be of length 9, and it should return 2 elements. 
The first element should be a tuple with 2 floats: the first element being the score you expect player 0 will get at the end of the game, and the second element being the score you expect player 1 will get at the end of the game.
The second element should be a dictionary of any important intermediate values that you used to calculate the scores.
For example, if you think player 0 will win 12 total points by the end of the game and player 1 will win 8 total points, the function should return (12, 8).\\

Make sure your output only includes the code of the function itself in plain text such that it is executable using exec() in python. Any helper functions should be defined within the scope of the function `evaluate state'.
Include comments in your code so that it is readable, but everything should be implemented. \\

The signature of the function should be as follows:

\begin{lstlisting}[language=Python, breaklines=true]
def evaluate_state(state) -> tuple[tuple[float, float], dict]:
    score_cards = state[0] # a python list of the score cards (integers) that have been played, in the order they were played
    player_0_played_cards = state[1] # a python list of the cards (integers) player 0 has played, in the order they were played. 
    player_1_played_cards = state[2] # a python list of the cards (integers) player 1 has played, in the order they were played. 
    is_turn = state[3] # bool, true if it is you and your opponent's turn to play, false if it is time to draw a new score card
    player_0_score = state[4] # float or integer, player 0's score so far
    player_1_score = state[5] #  float or integer, player 1's score so far
    score_deck = state[6] # a python set of the score cards (integers) left in the deck, either same length as player_0_hand and player_1_hand or one less since the score card appears before the players play. May be empty
    player_0_hand = state[7] # a python set of the cards (integers) left in player 0's hand. May be empty
    player_1_hand = state[8] # a python set of the cards (integers) left in player 1's hand. May be empty
    # explanation of what we do next
    ...
    <intermediate_value1> = value1 
    # explanation of what we do next
    ...
    <intermediate_value2> = value2 
    # explanation of what we do next
    ...
    player_scores = (player_0_expected_score, player_1_expected_score)
    intermediate_values = {'<intermediate_value1>': intermediate_value1, '<intermediate_value2>': intermediate_value2, ...}
    return player_scores, intermediate_values # make sure the return is exactly in this format
\end{lstlisting}
Where you can use your own names for the intermediate values and the values themselves.
Please start with "def evaluate state(state):"
\end{tcolorbox}

\subsection{Idea Generation Examples}

% \begin{tcolorbox}[colframe=custom3, colback=white, title=Prompt for idea generation]
% \texttt{<System prompt>}\\
% \texttt{<Game rules>}\\
% You previously generated the following section of the strategy guide: \\
% \texttt{<Previous guide>}\\
% Here is a possible way to improve your guide: \\
% \texttt{<Feedback reflections>}\\
% \end{tcolorbox}

The idea generation prompt included system prompt, game rules, previous guide and feedback reflections. Following those four components, we construct the format and an example of ideas to guide the generation of LLM.

\begin{tcolorbox}[colback=white,colframe=custom3,title=Prompt for idea generation]
\texttt{<System prompt>}\\
\texttt{<Game rules>}\\
\texttt{<Previous guide>}\\
\texttt{<Feedback reflections>}\\

Based on the function, feedback, and conclusions you drew, what are 2 improvements that you can make to the function that you think will have the most impact? Be as specific and concrete as possible, and write them out in the following format: \\

\begin{itemize}

  \item Thoughts: <your thoughts here>

  \item Idea 1: <your idea here>

  \item Idea 2: <your idea here>

\end{itemize}

...

Here's an example of what this might look like for 3 improvement ideas:

\begin{itemize}

  \item Thoughts: I should consider the number of cards left in the deck when evaluating the value of a state.

  \item Idea 1: I should add a term to the value function that penalizes states where there are fewer cards left in the deck.

  \item Idea 2: I should add a term to the value function that rewards states where the player has more cards in their hand than the opponent.

  \item Idea 3: I should add a term to the value function that rewards states where the player has more cards in their hand than the opponent and there are fewer cards left in the deck.

\end{itemize}

\end{tcolorbox}

Below is an instance of Feedback of GOPS game, showing the setup of two players, the intermediate values involved in the computation, and the actual scores.
\begin{tcolorbox}[colframe=black, title=Feedback example, colback=white]

Example 9: \\

The state you were trying to estimate a value for is: \\

The current state of the game is as follows:

\begin{itemize}

\item The score cards that have been revealed are: (2, 4, 5, 1, 3)

\item The cards that player 0 has played are: (1, 2, 4, 3, 5)

\item The cards that player 1 has played are: (3, 5, 1, 2, 4)

\item Player 0's score so far is: 9

\item Player 1's score so far is: 6

\item The score cards left in the deck are: set()

\item The cards left in player 0's hand are: set()

\item The cards left in player 1's hand are: set()

\end{itemize}

The function you generated returned the following values: \\

\{0: 3, 1: -3\} \\

for the expected end of game scores of the players.\\

Some intermediate values that you used to calculate the scores were: \\

\{'player\_0\_expected\_score': 9, 'player\_1\_expected\_score': 6, 'dynamic\_penalty': 0.0, 'player\_0\_hand\_reward': 0, 'player\_1\_hand\_reward': 0, 'player\_0\_adjustment': 0, 'player\_1\_adjustment': 0, 'player\_0\_strategic\_adjustment': 0, 'player\_1\_strategic\_adjustment': 0\} \\

The estimated end of game scores of the players using lookahead search with your function was: \\

\{0: 0.0, 1: 0.0\} \\

The actual scores of the players at the end of the game in the simulation were: \\

\{0: 3.0, 1: -3.0\} 

\end{tcolorbox}

Recall that feedback reflection refers to feedback for strategy, which is used to generate ideas. For prompting, We specify that game rules, previous guide and feedback examples are generated previously. The following is the prompt for feedback reflections.

\begin{tcolorbox}[colframe=custom5, colback=white, title=Prompt for feedback reflections]
\texttt{<System prompt>}\\
\texttt{<Game rules>}\\
Previously you generated the following function to evaluate the value of a state in the game.
\texttt{<Previous guide>}\\
Below is some feedback on how the function you generated performed when we tested it. Note that simulations involve high variance and the actual scores may not match the expected scores exactly. Hence, you should focus on trying to get the scores produced by your function to match those predicted by look-ahead search as closely as possible. 

\texttt{<Feedback examples>}\\
Based on the feedback given and the function you generated previously, what are some conclusions you can draw from the feedback? Make sure to cite the specific examples in the feedback to justify your analysis.
 \end{tcolorbox}

Below is the feedback reflections from the LLM.
\begin{tcolorbox}[colback=white,colframe=custom4,title=Feedback reflections]

From the feedback provided, we can draw several conclusions regarding the performance of the function in evaluating the value of a state in the GOPS game:\\

1. \textbf{Discrepancy in Expected Scores}: In several examples (e.g., Example 4, Example 7, Example 8), the expected end-of-game scores returned by the function do not match the scores predicted by look-ahead search closely. This indicates that the function may not be accurately estimating the value of the states in the game.\\

2. \textbf{Inconsistencies in Strategic Adjustments}: The function includes a strategic adjustment based on the opponent's played cards, but in all cases, the strategic adjustments are zero. This suggests that the strategic adjustments made in the function may not be capturing the true strategic implications of the opponent's moves effectively.\\

3. \textbf{Dynamic Penalty Adjustment}: The function includes a dynamic penalty adjustment based on the remaining high-value score cards in the deck. However, the dynamic penalty adjustments may not be accurately reflecting the impact of high-value score cards left in the deck on the game outcome.\\

4. \textbf{Limited Hand Size Reward}: The function rewards states where a player has more cards in their hand than the opponent. While this reward is included, it might not be capturing the full strategic implications of having more cards in hand effectively.\\

5. \textbf{Simulation vs. Expected Scores}: The actual scores at the end of the game in the simulations do not match the expected scores returned by the function precisely. This indicates that the function's evaluation may not be aligning well with the actual game outcomes.\\

In conclusion, the function may need further refinement in terms of capturing strategic adjustments, dynamic penalties, and hand size rewards to improve the accuracy of the state evaluation in the GOPS game. Additionally, considering the discrepancies between the expected and actual scores, further testing and adjustments may be necessary to enhance the function's performance in evaluating the value of states accurately.

\end{tcolorbox}

Also, with the prompts of idea generation, below is the generated new ideas by LLM.

\begin{tcolorbox}[colframe=custom4, colback=white, title=Generated new ideas]
Thoughts: The function needs to better capture the strategic implications of the opponent's moves and adjust the expected scores accordingly. Additionally, the dynamic penalty adjustment and hand size rewards could be improved to better reflect their impact on the game outcome.\\

Idea 1: Enhance the strategic adjustment component of the function by analyzing the opponent's played cards more deeply. This could involve considering patterns in the opponent's moves, potential card combinations, and predicting future moves based on past actions.\\

Idea 2: Revise the dynamic penalty adjustment to more accurately reflect the impact of high-value score cards left in the deck. This could involve adjusting the penalty dynamically based on the remaining high-value cards and their likelihood of being drawn in future rounds. This adjustment could help in better assessing the risk associated with certain states in the game.\\
\end{tcolorbox}

\subsection{Strategy Implementation Examples}
\label{sec:vh_strategy_examples}
During the strategy implementation step, we first select a strategy and an idea from the libraries using the adaptive selection policy. Then, we prompt the LLM to implement the idea on the strategy, generating a new improved strategy. 

In this section, we showcase two examples. Each example illustrates strategies before and after enhancements made by the LLM. This comparison highlights the effectiveness of our strategy implementation. The improved parts by LLM are highlighted in yellow.

Below is the prompt for strategy implementation.

\begin{tcolorbox}[colframe=custom3, colback=white, title=Prompt for implementation]
\texttt{<System prompt>}\\
\texttt{<Game rules>}\\
Previously you generated the following function to evaluate the value of a state in the game: \\
\texttt{<Previous guide>}\\
Here is a possible way to improve this function:  \\
\texttt{<Improvement ideas>}\\
\end{tcolorbox}

\subsubsection{Example 1}
Below is the GOPS Value Heuristics Function before the strategy improvement.
\begin{tcolorbox}[title=GOPS Value Heuristics Function (Before), colback=white, colframe=custom6]
\begin{lstlisting}[language=Python, breaklines=true]
def evaluate_state(state) -> tuple[tuple[float, float], dict]:
    score_cards = state[0]
    player_0_played_cards = state[1]
    player_1_played_cards = state[2]
    is_turn = state[3]
    player_0_score = state[4]
    player_1_score = state[5]
    score_deck = state[6]
    player_0_hand = state[7]
    player_1_hand = state[8]
    
    # Calculate the potential scores for each player based on the remaining score cards
    player_potential_score = player_0_score
    opponent_potential_score = player_1_score
    
    if len(score_deck) > 0:
        remaining_score_cards = len(score_deck)
        if len(player_0_played_cards) > len(player_1_played_cards):
            player_potential_score += remaining_score_cards / 2
        elif len(player_1_played_cards) > len(player_0_played_cards):
            opponent_potential_score += remaining_score_cards / 2
    
    player_advantage = player_potential_score - opponent_potential_score
    
    return (player_potential_score, opponent_potential_score), {'player_advantage': player_advantage}
\end{lstlisting}
\end{tcolorbox}

Below is the selected idea to improve the above strategy.
\begin{tcolorbox}[title=Selected GOPS Value Heuristics Improvement Idea, colback=white, colframe=custom5]
Update the function to calculate the advantage of winning future rounds based on the potential scores each player could achieve with the remaining score cards and their current scores. This would involve considering the number of cards left in the deck, the players' hands, and the current scores to determine the advantage one player may have over the other in the upcoming rounds.
\end{tcolorbox}

Below is the GOPS Value Heuristics Function after enhancement by LLM.
The improved parts by LLM are highlighted in yellow.

% \begin{highlighted}[title=GOPS Value Heuristics Function (After)]
\begin{tcolorbox}[title=GOPS Value Heuristics Function (After), colback=white, colframe=custom4]
\begin{lstlisting}[language=Python, breaklines=true, escapechar=@]
def evaluate_state(state) -> tuple[tuple[float, float], dict]:
    score_cards = state[0] 
    player_0_played_cards = state[1] 
    player_1_played_cards = state[2] 
    is_turn = state[3] 
    player_0_score = state[4] 
    player_1_score = state[5] 
    score_deck = state[6] 
    player_0_hand = state[7] 
    player_1_hand = state[8] 
    
    # Calculate the potential scores for each player based on the remaining score cards 
    # and current scores
    player_potential_score = player_0_score + sum(score_deck) / 2
    opponent_potential_score = player_1_score + sum(score_deck) / 2
    
    # Determine the advantage of winning future rounds based on potential score
    @\Hilight@if is_turn:
    @\Hilight@    player_potential_scores = [player_potential_score + card for card in player_0_hand]
    @\Hilight@    opponent_potential_scores = [opponent_potential_score + card for card in player_1_hand]
        
    @\Hilight@    player_advantage = sum(player_potential_scores) / len(player_potential_scores) 
    @\Hilight@    - sum(opponent_potential_scores) / len(opponent_potential_scores)
    @\Hilight@else:
    @\Hilight@    player_advantage = player_potential_score - opponent_potential_score
    
    return (player_potential_score, opponent_potential_score), {'player_advantage': player_advantage}
\end{lstlisting}
\end{tcolorbox}
% \end{highlighted}

\subsubsection{Example 2}
Below is the Avalon Value Heuristics Function before improvements.
\begin{tcolorbox}[title=Avalon Value Heuristics Function (Before), colback=white,colframe=custom6]
 % players = state['players']
 %    turn = state['turn']
 %    phase = state['phase']
 %    round_number = state['round']
 %    quest_leader = state['quest_leader']
 %    quest_team = state['quest_team']
 %    historical_quest_results = state['historical_quest_results']
 %    historical_team_votes = state['historical_team_votes']
 %    num_good = state['num_good']
 %    num_participants_per_quest = state['num_participants_per_quest']
 %    num_fails_per_quest = state['num_fails_per_quest']
 %    roles = state['roles']
 %    is_good = state['is_good']
\begin{lstlisting}[language=Python, breaklines=true]

def evaluate_state(state):
    num_successful_quests = sum(historical_quest_results)
    num_failed_quests = len(historical_quest_results) - num_successful_quests
    num_remaining_quests = len(num_participants_per_quest) - len(historical_quest_results)

    num_evil = len(players) - num_good
    num_evil_in_quest_team = len([player for player in quest_team if not is_good[player]])

    success_probability = 0.5
    if phase == 0: 
        if num_successful_quests >= 3:
            success_probability = 0.9
        elif num_failed_quests >= 3:
            success_probability = 0.1
    elif phase == 1: 
        success_probability = 0.8 if num_evil_in_quest_team == 0 else 0.2
    elif phase == 2: 
        success_probability = 0.9 if num_successful_quests > num_failed_quests else 0.1
    elif phase == 3: 
        if 'Merlin' in roles and 'Assassin' in roles:
            merlin_index = roles.index('Merlin')
            assassin_index = roles.index('Assassin')
            if assassin_index in quest_team:
                success_probability = 0.1
            else:
                success_probability = 0.9 

    expected_winrates_per_player = dict()
    for player in players:
        if is_good[player]:
            expected_winrates_per_player[player] = success_probability
        else:
            expected_winrates_per_player[player] = 1 - success_probability

    intermediate_values = {
        'num_successful_quests': num_successful_quests,
        'num_failed_quests': num_failed_quests,
        'num_remaining_quests': num_remaining_quests,
        'num_evil_in_quest_team': num_evil_in_quest_team
    }

    return expected_winrates_per_player, intermediate_values
\end{lstlisting}
\end{tcolorbox}

Below is the improvement idea pf Avalon Value Heuristics Function.
\begin{tcolorbox}[title=Avalon Value Heuristics Function Improvement Idea, colback=white,colframe=custom5]
Incorporate a more nuanced success probability calculation based on the roles of the players and the current phase of the game. For example, in phase 1 (team selection), consider the balance of Good and Evil players on the quest team and adjust the success probability accordingly. This can help better reflect the strategic considerations during team selection.
\end{tcolorbox}

The following is Avalon Value Heuristics Function after enhancements, highlighted in yellow.
\begin{tcolorbox}[title=Avalon Value Heuristics Function (After), colback=white,colframe=custom4]
% players: set[int] = state['players']
%     turn: int = state['turn']
%     phase: int = state['phase']
%     round_number: int = state['round']
%     quest_leader: int = state['quest_leader']
%     quest_team: set[int] = state['quest_team']
%     historical_quest_results: list[bool] = state['historical_quest_results']
%     historical_team_votes: list[bool] = state['historical_team_votes']
%     num_good: int = state['num_good']
%     num_participants_per_quest: list[int] = state['num_participants_per_quest']
%     num_fails_per_quest: list[int] = state['num_fails_per_quest']
%     roles: list[str] = state['roles']
%     is_good: list[bool] = state['is_good']
\begin{lstlisting}[language=Python, breaklines=true, escapechar=@]
def evaluate_state(state: dict) -> tuple[dict[int, float], dict]:
    
    prob_good_victory = 0.5  # probability that Good will win

    if phase == 0:  # team selection phase
    @\Hilight@    num_successful_quests = sum(historical_quest_results)
    @\Hilight@    num_failed_quests = len(historical_quest_results) - num_successful_quests
    @\Hilight@    num_remaining_quests = len(num_participants_per_quest) - len(historical_quest_results)
    @\Hilight@    num_evil = len(players) - num_good
    @\Hilight@    num_evil_in_quest_team = len([player for player in quest_team if not is_good[player]])

        if num_successful_quests >= 3:
            prob_good_victory = 0.9
        elif num_failed_quests >= 3:
            prob_good_victory = 0.1

    @\Hilight@    intermediate_value1 = {'num_successful_quests': num_successful_quests, 'num_failed_quests': num_failed_quests,
                               'num_remaining_quests': num_remaining_quests}
    @\Hilight@    intermediate_value2 = {'num_evil_in_quest_team': num_evil_in_quest_team}

    elif phase == 1:  # team approval phase
        num_evil_in_quest_team = len([player for player in quest_team if not is_good[player]])

        prob_good_victory = 0.8 if num_evil_in_quest_team == 0 else 0.2

    @\Hilight@    intermediate_value1 = {'num_evil_in_quest_team': num_evil_in_quest_team}
    @\Hilight@    intermediate_value2 = {}  # Initialize empty dictionary to avoid the error

    elif phase == 2:  # quest phase
        num_successful_quests = sum(historical_quest_results)
        num_failed_quests = len(historical_quest_results) - num_successful_quests

        prob_good_victory = 0.9 if num_successful_quests > num_failed_quests else 0.1

    @\Hilight@    intermediate_value1 = {'num_successful_quests': num_successful_quests, 'num_failed_quests': num_failed_quests}
    @\Hilight@    intermediate_value2 = {}  # Initialize empty dictionary to avoid the error
\end{lstlisting}
\end{tcolorbox}

\begin{tcolorbox}[ colback=white,colframe=custom6]
% players: set[int] = state['players']
%     turn: int = state['turn']
%     phase: int = state['phase']
%     round_number: int = state['round']
%     quest_leader: int = state['quest_leader']
%     quest_team: set[int] = state['quest_team']
%     historical_quest_results: list[bool] = state['historical_quest_results']
%     historical_team_votes: list[bool] = state['historical_team_votes']
%     num_good: int = state['num_good']
%     num_participants_per_quest: list[int] = state['num_participants_per_quest']
%     num_fails_per_quest: list[int] = state['num_fails_per_quest']
%     roles: list[str] = state['roles']
%     is_good: list[bool] = state['is_good']
\begin{lstlisting}[language=Python, breaklines=true, escapechar=@]
    elif phase == 3:  # assassination phase
        merlin_index = roles.index('Merlin')
        assassin_index = roles.index('Assassin')

        if assassin_index in quest_team:
            prob_good_victory = 0.1
        else:
            prob_good_victory = 0.9

    @\Hilight@intermediate_value1 = {'merlin_index': merlin_index, 'assassin_index': assassin_index}
    @\Hilight@intermediate_value2 = {}  # Initialize empty dictionary to avoid the error

    expected_winrates_per_player = dict()
    prob_evil_victory = 1 - prob_good_victory
    for player in players:
        if is_good[player]:
            expected_winrates_per_player[player] = prob_good_victory
        else:
            expected_winrates_per_player[player] = prob_evil_victory

    @\Hilight@intermediate_values = {'intermediate_value1': intermediate_value1, 'intermediate_value2': intermediate_value2}

    return expected_winrates_per_player, intermediate_values
\end{lstlisting}
\end{tcolorbox}

% % \subsection{Seed function generation}

\subsubsection{Example 3}
Below is the GOPS Value Heuristics Function before the strategy improvement.

\begin{tcolorbox}[title=GOPS Value Heuristics Function (Before), colback=white, colframe=custom6]
\begin{lstlisting}[language=Python, breaklines=true]
def evaluate_state(state) -> tuple[tuple[float, float], dict]:
    score_cards = state[0]
    player_0_played_cards = state[1]
    player_1_played_cards = state[2]
    is_turn = state[3]
    player_0_score = state[4]
    player_1_score = state[5]
    score_deck = state[6]
    player_0_hand = state[7]
    player_1_hand = state[8]

    # Calculate initial potentials
    player_0_potential = sum(player_0_hand)
    player_1_potential = sum(player_1_hand)
    score_potential = sum(score_deck)

    # Update player potentials based on remaining cards and score deck
    player_0_potential += sum(card for card in player_0_hand if any(card > score for score in score_deck))
    player_1_potential += sum(card for card in player_1_hand if any(card > score for score in score_deck))

    # Add half of the score potential to the player who has the turn
    if is_turn:
        player_0_potential += score_potential / 2
    else:
        player_1_potential += score_potential / 2

    # Count the number of certain wins for each player
    player_0_certain_wins = sum(card > max(player_1_hand) for card in player_0_hand)
    player_1_certain_wins = sum(card > max(player_0_hand) for card in player_1_hand)

    rounds_left = len(score_deck)

    # Dynamic adjustment based on specific cards played
    player_0_certain_wins_adjust = 0
    player_1_certain_wins_adjust = 0
    for i in range(len(player_0_played_cards)):
        if player_0_played_cards[i] > player_1_played_cards[i]:
            player_0_certain_wins_adjust += 1
        elif player_1_played_cards[i] > player_0_played_cards[i]:
            player_1_certain_wins_adjust += 1
    
    player_0_certain_wins += player_0_certain_wins_adjust
    player_1_certain_wins += player_1_certain_wins_adjust

    # Add potential scores from certain wins
    if rounds_left <= player_0_certain_wins:
        highest_scores = sorted(score_deck)[-rounds_left:]
        player_0_potential += sum(highest_scores)
        
    if rounds_left <= player_1_certain_wins:
        highest_scores = sorted(score_deck)[-rounds_left:]
        player_1_potential += sum(highest_scores)
\end{lstlisting}
\end{tcolorbox}
\begin{tcolorbox}[ colback=white,colframe=custom6]
\begin{lstlisting}[language=Python, breaklines=true, escapechar=@]
    # Calculate expected scores
    player_0_expected_score = player_0_score + player_0_potential
    player_1_expected_score = player_1_score + player_1_potential

    # Calculate the difference in the sum of played cards
    sum_player_0_played_cards = sum(player_0_played_cards)
    sum_player_1_played_cards = sum(player_1_played_cards)
    sum_played_cards_diff = sum_player_0_played_cards - sum_player_1_played_cards

    # Adjust scores based on the difference in the sum of played cards
    adjustment_factor = 0.1  # Adjust this factor based on the level of adjustment desired
    player_0_expected_score += sum_played_cards_diff * adjustment_factor
    player_1_expected_score -= sum_played_cards_diff * adjustment_factor

    # Dynamic adjustment based on uncertainty in the game state
    uncertainty_factor = 0.1 * rounds_left  # Adjust this factor based on the level of uncertainty desired
    player_0_expected_score += player_0_potential * uncertainty_factor
    player_1_expected_score += player_1_potential * uncertainty_factor

    # Refine uncertainty factor based on specific conditions
    if len(player_0_hand) == 1:
        uncertainty_factor *= 0.5
    if len(player_1_hand) == 1:
        uncertainty_factor *= 0.5

    # Store intermediate values in a dictionary
    intermediate_values = {
        'player_0_potential': player_0_potential,
        'player_1_potential': player_1_potential,
        'score_potential': score_potential,
        'player_0_certain_wins': player_0_certain_wins,
        'player_1_certain_wins': player_1_certain_wins,
        'player_0_certain_wins_adjust': player_0_certain_wins_adjust,
        'player_1_certain_wins_adjust': player_1_certain_wins_adjust,
        'sum_played_cards_diff': sum_played_cards_diff,
        'uncertainty_factor': uncertainty_factor
    }

    return (player_0_expected_score, player_1_expected_score), intermediate_values
\end{lstlisting}
\end{tcolorbox}

Below is the selected idea to improve the above strategy.

\begin{tcolorbox}[title=Selected GOPS Value Heuristics Improvement Idea, colback=white, colframe=custom5]

Incorporate a term in the value function that takes into account the distribution of score cards left in the deck. Certain score cards may have a higher value or strategic importance, so adjusting the potentials based on the presence of these cards can provide a more accurate evaluation of the state.

\end{tcolorbox}

Below is the GOPS Value Heuristics Function after enhancement by LLM. The improved parts by LLM are highlighted in yellow.

\begin{tcolorbox}[title=GOPS Value Heuristics Function (After), colback=white, colframe=custom4]
\begin{lstlisting}[language=Python, breaklines=true, escapechar=@]
def evaluate_state(state) -> tuple[tuple[float, float], dict]:
    score_cards = state[0]
    player_0_played_cards = state[1]
    player_1_played_cards = state[2]
    is_turn = state[3]
    player_0_score = state[4]
    player_1_score = state[5]
    score_deck = state[6]
    player_0_hand = state[7]
    player_1_hand = state[8]

    # Calculate initial potentials
    player_0_potential = sum(player_0_hand)
    player_1_potential = sum(player_1_hand)
    score_potential = sum(score_deck)

    # Update player potentials based on remaining cards and score deck
    player_0_potential += sum(card for card in player_0_hand if any(card > score for score in score_deck))
    player_1_potential += sum(card for card in player_1_hand if any(card > score for score in score_deck))

    # Add half of the score potential to the player who has the turn
    if is_turn:
        player_0_potential += score_potential / 2
    else:
        player_1_potential += score_potential / 2

    # Count the number of certain wins for each player
    player_0_certain_wins = sum(card > max(player_1_hand) for card in player_0_hand)
    player_1_certain_wins = sum(card > max(player_0_hand) for card in player_1_hand)

    rounds_left = len(score_deck)

    # Dynamic adjustment based on specific cards played
    player_0_certain_wins_adjust = 0
    player_1_certain_wins_adjust = 0
    for i in range(len(player_0_played_cards)):
        if player_0_played_cards[i] > player_1_played_cards[i]:
            player_0_certain_wins_adjust += 1
        elif player_1_played_cards[i] > player_0_played_cards[i]:
            player_1_certain_wins_adjust += 1
    
    player_0_certain_wins += player_0_certain_wins_adjust
    player_1_certain_wins += player_1_certain_wins_adjust

    # Add potential scores from certain wins
    if rounds_left <= player_0_certain_wins:
        highest_scores = sorted(score_deck)[-rounds_left:]
        player_0_potential += sum(highest_scores)
        
    if rounds_left <= player_1_certain_wins:
        highest_scores = sorted(score_deck)[-rounds_left:]
        player_1_potential += sum(highest_scores)

    @\Hilight@ # Incorporate distribution of score cards left in the deck
    @\Hilight@ important_score_cards = {7, 10, 13}  # Example: define important score cards
    @\Hilight@ player_0_potential += sum(card for card in player_0_hand if card in important_score_cards)
    @\Hilight@ player_1_potential += sum(card for card in player_1_hand if card in important_score_cards)

    # Calculate expected scores
    player_0_expected_score = player_0_score + player_0_potential
    player_1_expected_score = player_1_score + player_1_potential

    # Calculate the difference in the sum of played cards
    sum_player_0_played_cards = sum(player_0_played_cards)
    sum_player_1_played_cards = sum(player_1_played_cards)
    sum_played_cards_diff = sum_player_0_played_cards - sum_player_1_played_cards
\end{lstlisting}
\end{tcolorbox}
\begin{tcolorbox}[ colback=white,colframe=custom6]
\begin{lstlisting}[language=Python, breaklines=true, escapechar=@]
    # Adjust scores based on the difference in the sum of played cards
    adjustment_factor = 0.1  # Adjust this factor based on the level of adjustment desired
    player_0_expected_score += sum_played_cards_diff * adjustment_factor
    player_1_expected_score -= sum_played_cards_diff * adjustment_factor

    # Dynamic adjustment based on uncertainty in the game state
    uncertainty_factor = 0.1 * rounds_left  # Adjust this factor based on the level of uncertainty desired
    player_0_expected_score += player_0_potential * uncertainty_factor
    player_1_expected_score += player_1_potential * uncertainty_factor

    # Refine uncertainty factor based on specific conditions
    if len(player_0_hand) == 1:
        uncertainty_factor *= 0.5
    if len(player_1_hand) == 1:
        uncertainty_factor *= 0.5

    # Store intermediate values in a dictionary
    intermediate_values = {
        'player_0_potential': player_0_potential,
        'player_1_potential': player_1_potential,
        'score_potential': score_potential,
        'player_0_certain_wins': player_0_certain_wins,
        'player_1_certain_wins': player_1_certain_wins,
        'player_0_certain_wins_adjust': player_0_certain_wins_adjust,
        'player_1_certain_wins_adjust': player_1_certain_wins_adjust,
        'sum_played_cards_diff': sum_played_cards_diff,
        'uncertainty_factor': uncertainty_factor
    }

    return (player_0_expected_score, player_1_expected_score), intermediate_values
\end{lstlisting}
\end{tcolorbox}

\subsubsection{Example 4}
Below is the GOPS Value Heuristics Function before the strategy improvement.

\begin{tcolorbox}[title=GOPS Value Heuristics Function (Before), colback=white, colframe=custom6]
\begin{lstlisting}[language=Python, breaklines=true]
def evaluate_state(state) -> tuple[tuple[float, float], dict]:
    score_cards = state[0]
    player_0_played_cards = state[1]
    player_1_played_cards = state[2]
    is_turn = state[3]
    player_0_score = state[4]
    player_1_score = state[5]
    score_deck = state[6]
    player_0_hand = state[7]
    player_1_hand = state[8]

    # Calculate initial potentials
    player_0_potential = sum(player_0_hand)
    player_1_potential = sum(player_1_hand)
    score_potential = sum(score_deck)

    # Add half of the score potential to the player who has the turn
    if is_turn:
        player_0_potential += score_potential / 2
    else:
        player_1_potential += score_potential / 2

    # Count the number of certain wins for each player
    player_0_certain_wins = sum(card > max(player_1_hand) for card in player_0_hand)
    player_1_certain_wins = sum(card > max(player_0_hand) for card in player_1_hand)

    rounds_left = len(score_deck)

    # Add potential scores from certain wins
    if rounds_left <= player_0_certain_wins:
        highest_scores = sorted(score_deck)[-rounds_left:]
        player_0_potential += sum(highest_scores)
        
    if rounds_left <= player_1_certain_wins:
        highest_scores = sorted(score_deck)[-rounds_left:]
        player_1_potential += sum(highest_scores)

    # New improvement: Incorporate a probabilistic approach based on the remaining score cards
    player_0_expected_score = player_0_score + player_0_potential
    player_1_expected_score = player_1_score + player_1_potential

    # Dynamic evaluation of opponent's potential moves
    opponent_potential = sum(player_0_hand) if is_turn else sum(player_1_hand)
    opponent_certain_wins = sum(card > max(player_1_hand) for card in player_0_hand) if is_turn else sum(card > max(player_0_hand) for card in player_1_hand)

    # Adjust evaluation based on opponent's potential plays
    if rounds_left <= opponent_certain_wins:
        highest_scores = sorted(score_deck)[-rounds_left:]
        if is_turn:
            player_1_potential += sum(highest_scores)
        else:
            player_0_potential += sum(highest_scores)

    # Store intermediate values in a dictionary
    intermediate_values = {
        'player_0_potential': player_0_potential,
        'player_1_potential': player_1_potential,
        'score_potential': score_potential,
        'player_0_certain_wins': player_0_certain_wins,
        'player_1_certain_wins': player_1_certain_wins,
        'opponent_potential': opponent_potential,
        'opponent_certain_wins': opponent_certain_wins,
        'player_0_expected_score': player_0_expected_score,
        'player_1_expected_score': player_1_expected_score
    }

    return (player_0_expected_score, player_1_expected_score), intermediate_values
\end{lstlisting}
\end{tcolorbox}

Below is the selected idea to improve the above strategy.

\begin{tcolorbox}[title=Selected GOPS Value Heuristics Improvement Idea, colback=white, colframe=custom5]

Introduce a penalty factor for potential scores that are excessively high, indicating potential overestimation. By capping the potential scores or applying a scaling factor based on certain thresholds, we can prevent the function from assigning unrealistic values and improve the accuracy of the value heuristic.

\end{tcolorbox}

Below is the GOPS Value Heuristics Function after enhancement by LLM. The improved parts by LLM are highlighted in yellow.

\begin{tcolorbox}[title=GOPS Value Heuristics Function (After), colback=white, colframe=custom4]
\begin{lstlisting}[language=Python, breaklines=true, escapechar=@]

def evaluate_state(state) -> tuple[tuple[float, float], dict]:
    score_cards = state[0]
    player_0_played_cards = state[1]
    player_1_played_cards = state[2]
    is_turn = state[3]
    player_0_score = state[4]
    player_1_score = state[5]
    score_deck = state[6]
    player_0_hand = state[7]
    player_1_hand = state[8]

    # Calculate initial potentials
    player_0_potential = sum(player_0_hand)
    player_1_potential = sum(player_1_hand)
    score_potential = sum(score_deck)

    # Add half of the score potential to the player who has the turn
    if is_turn:
        player_0_potential += score_potential / 2
    else:
        player_1_potential += score_potential / 2

    # Count the number of certain wins for each player
    player_0_certain_wins = sum(card > max(player_1_hand) for card in player_0_hand)
    player_1_certain_wins = sum(card > max(player_0_hand) for card in player_1_hand)

    rounds_left = len(score_deck)

    # Add potential scores from certain wins
    if rounds_left <= player_0_certain_wins:
        highest_scores = sorted(score_deck)[-rounds_left:]
        player_0_potential += sum(highest_scores)
        
    if rounds_left <= player_1_certain_wins:
        highest_scores = sorted(score_deck)[-rounds_left:]
        player_1_potential += sum(highest_scores)


    
\end{lstlisting}
\end{tcolorbox}

\begin{tcolorbox}[ colback=white,colframe=custom6]
\begin{lstlisting}[language=Python, breaklines=true, escapechar=@]

    # New improvement: Incorporate a probabilistic approach based on the remaining score cards
    player_0_expected_score = player_0_score + player_0_potential
    player_1_expected_score = player_1_score + player_1_potential

    # Dynamic evaluation of opponent's potential moves
    opponent_potential = sum(player_0_hand) if is_turn else sum(player_1_hand)
    opponent_certain_wins = sum(card > max(player_1_hand) for card in player_0_hand) if is_turn else sum(card > max(player_0_hand) for card in player_1_hand)

    # Adjust evaluation based on opponent's potential plays
    if rounds_left <= opponent_certain_wins:
        highest_scores = sorted(score_deck)[-rounds_left:]
        if is_turn:
            player_1_potential += sum(highest_scores)
        else:
            player_0_potential += sum(highest_scores)

    @\Hilight@ # Introduce a penalty factor for excessively high potential scores
    @\Hilight@ penalty_threshold = 100  # Define a threshold for potential scores to trigger penalty
    @\Hilight@ penalty_factor = 0.5  # Define a factor by which to reduce potential scores above threshold

    @\Hilight@ if player_0_potential > penalty_threshold:
    @\Hilight@    player_0_potential = penalty_threshold + (player_0_potential - penalty_threshold) * 
    @\Hilight@      penalty_factor

    @\Hilight@ if player_1_potential > penalty_threshold:
    @\Hilight@    player_1_potential = penalty_threshold + (player_1_potential - penalty_threshold) * 
    @\Hilight@      penalty_factor

    # Store intermediate values in a dictionary
    intermediate_values = {
        'player_0_potential': player_0_potential,
        'player_1_potential': player_1_potential,
        'score_potential': score_potential,
        'player_0_certain_wins': player_0_certain_wins,
        'player_1_certain_wins': player_1_certain_wins,
        'opponent_potential': opponent_potential,
        'opponent_certain_wins': opponent_certain_wins,
        'player_0_expected_score': player_0_expected_score,
        'player_1_expected_score': player_1_expected_score
    }

    return (player_0_expected_score, player_1_expected_score), intermediate_values
    
\end{lstlisting}
\end{tcolorbox}
