# Supplementary material for: PIANIST: Learning Partially Observable World Models with LLMs for Multi-Agent Decision Making
Source: arXiv:2411.15998 source file (2024-11-24)
Supplement: Supplementary file 12 [file exp_compute_src.tex]

\section{Experimental Compute Resources}
\label{append_exp_comput_src}

All experiments in this work were performed on a workstation with an NVIDIA GeForce RTX 3070 GPU, Intel Core i9-10900 CPU at 2.80 GHz, and a Macbook Pro.
