# Supplementary material for: PIANIST: Learning Partially Observable World Models with LLMs for Multi-Agent Decision Making
Source: arXiv:2411.15998 source file (2024-11-24)
Supplement: Supplementary file 13 [file significance_tests.tex]

\section{Significance tests}
\label{sec:significance_tests}

\subsection{Table \ref{tab:evolver}}
The one-way ANOVA test indicates a statistically significant difference between the means of \method and the other groups for the game of GOPS shown in Table \ref{tab:evolver}, with a F-statistic of 29.49 and a p-value of approximately 
$2.61 \times 10^{-6}$. This suggests that \method has a mean that is significantly different from the means for the other improvement methods.\\

The one-way ANOVA test indicates a statistically significant difference between the means of \method and the other groups for the game of Avalon shown in Table \ref{tab:evolver}, with a F-statistic of 4.90 and a p-value of approximately 0.0026. This suggests that \method has a mean that is significantly different from the means for the other improvement methods.

\subsection{Table \ref{tab:feedback}}
The one-way ANOVA test for this data indicates a statistically significant difference between the means of \method and the other groups ('Critic' and 'Outcome'), with a F-statistic of 4.08 and a p-value of approximately 0.0299. This suggests that \method has a mean that is significantly different from the means of the other groups in this dataset.

\subsection{Figure \ref{fig:token_performance}}
