# Supplementary material for: PIANIST: Learning Partially Observable World Models with LLMs for Multi-Agent Decision Making
Source: arXiv:2411.15998 source file (2024-11-24)
Supplement: Supplementary file 14 [file vh_implementation.tex]

\section{Value Heuristic Implementation Details}
\label{vh_implementation}
