# Supplementary material for: PIANIST: Learning Partially Observable World Models with LLMs for Multi-Agent Decision Making
Source: arXiv:2411.15998 source file (2024-11-24)
Supplement: Supplementary file 15 [file temp.tex]

\section{LLM Example inputs and outputs}

\subsection{GOPS Value Heuristic}
\begin{tcolorbox}[title=GOPS value heuristic idea generation prompt,  colframe=blue]
  Placeholder
\end{tcolorbox}

\begin{tcolorbox}[title=GOPS value heuristic idea generation output,  colframe=blue]
  Placeholder
\end{tcolorbox}

\begin{tcolorbox}[title=GOPS value heuristic strategy implementation prompt,  colframe=blue]
  Placeholder
\end{tcolorbox}

\begin{tcolorbox}[title=GOPS value heuristic strategy implementation  output,  colframe=blue]
  Placeholder
\end{tcolorbox}

\subsection{Avalon Value Heuristic}

\begin{tcolorbox}[colback=white,colframe=black,title=Feedback]
\textbf{Example 16:}\\
The state you were trying to estimate a value for is:\\
\texttt{State((2, 2, 1, 0, False, (0, 2, 5), (1, 1, 1, 1, 0, 1), (1, 0), (False,), (7, 0, 5, 5, 6, 5), (0, 2, 5), ()), \{\})}\\
The function you generated returned the following values:\\
\{0: -0.4, 1: 0.3999999999999999, 2: 0.3999999999999999, 3: 0.3999999999999999, 4: -0.4, 5: 0.3999999999999999\}\\
for the expected end of game scores of the players.\\
Some intermediate values that you used to calculate the scores were:\\
\{'example\_value': 0.5\}\\
The estimated end of game scores of the players using lookahead search with your function was:\\
\{0: -0.39999999999745345, 1: 0.39999999999745334, 2: 0.39999999999745334, 3: 0.39999999999745334, 4: -0.39999999999745345, 5: 0.39999999999745334\}\\
The actual scores of the players at the end of the game in the simulation were:\\
\{0: 1.0, 1: -1.0, 2: -1.0, 3: -1.0, 4: 1.0, 5: -1.0\}\\

\textbf{Example 30:}\\
The state you were trying to estimate a value for is:\\
\texttt{State((3, 3, 3, 0, False, (1, 3, 4, 5), (1, 1, 1, 1, 1, 1), (1, 1, 1, 1), (True, True, True), (5, 7, 5, 5, 6, 0), (1,), ()), \{\})}\\
The function you generated returned the following values:\\
\{0: 0.3999999999999999, 1: -0.4, 2: 0.3999999999999999, 3: 0.3999999999999999, 4: -0.4, 5: 0.3999999999999999\}\\
for the expected end of game scores of the players.\\
Some intermediate values that you used to calculate the scores were:\\
\{'example\_value': 0.5\}\\
The estimated end of game scores of the players using lookahead search with your function was:\\
\{0: 0.0, 1: 0.0, 2: 0.0, 3: 0.0, 4: 0.0, 5: 0.0\}\\
The actual scores of the players at the end of the game in the simulation were:\\
\{0: 1.0, 1: -1.0, 2: 1.0, 3: 1.0, 4: -1.0, 5: 1.0\}\\

% Fill in the remaining examples using the same structure

\end{tcolorbox}

\begin{tcolorbox}[colback=white,colframe=black,title=Feedback conclusions dialogue]
From the feedback provided, it is evident that players in The Resistance: Avalon pay close attention to the behavior and statements made by each player during the discussion phase to determine their trustworthiness and potential role. In the example provided, Player 1, who claimed to be Merlin, emphasized their dedication to identifying Evil players and ensuring the success of the quests. This led to varying reactions from the other players, with some finding Player 1's speech convincing and aligned with the goals of Good, therefore increasing the probability of Player 1 being Merlin. However, there were also players who viewed Player 1's behavior as potentially strategic and an attempt to deflect suspicion from their true Evil identity, leading to an increase in the probability of Player 1 being Evil.\\

This feedback highlights the importance of not only stating one's intentions clearly during the discussion phase as Merlin but also ensuring that these statements are perceived as genuine and aligned with the goals of the Good team. Players should be strategic in their approach, balancing between gaining trust from other players and avoiding suspicion from the Evil team. Additionally, players should be mindful of how their behavior and statements may be interpreted by others, as perceptions can heavily influence the probability of being identified correctly as Merlin or Evil.\\

In conclusion, to play the Merlin role effectively during the discussion phase in The Resistance: Avalon, players should focus on emphasizing their dedication to identifying Evil players, ensuring the success of quests, and working together with the Good team. It is crucial to strike a balance between gaining trust and avoiding suspicion, as perceptions of one's behavior and statements can significantly impact how other players perceive their role in the game.
\end{tcolorbox}


\begin{tcolorbox}[title=Avalon value heuristic idea generation prompt,  colframe=blue]
\begin{verbatim}
def evaluate_state(state: dict) -> tuple[dict[Any, float], dict]:
    # Extract relevant information from the game state
    players = state['players']
    turn = state['turn']
    phase = state['phase']
    round = state['round']
    quest_leader = state['quest_leader']
    quest_team = state['quest_team']
    historical_quest_results = state['historical_quest_results']
    historical_team_votes = state['historical_team_votes']
    num_good = state['num_good']
    num_participants_per_quest = state['num_participants_per_quest']
    num_fails_per_quest = state['num_fails_per_quest']
    roles = state['roles']
    is_good = state['is_good']
    
    # Placeholder for intermediate values
    intermediate_values = {}
    
    # Calculate expected win rate for each player
    player_win_rates = {}
    
    # Sample calculation of win rates - replace with your own logic
    for player in players:
        if is_good[player]:
            # Example: Good players have a higher win rate
            player_win_rates[player] = 0.7
        else:
            # Example: Evil players have a lower win rate
            player_win_rates[player] = 0.3
    
    # Add intermediate values to the dictionary
    intermediate_values['example_value'] = 0.5
    
    return player_win_rates, intermediate_values
\end{verbatim}
\end{tcolorbox}

\begin{tcolorbox}[title=Avalon value heuristic idea generation prompt,  colframe=blue]

\texttt{SYS PROMPT}\\

\texttt{AVALON RULES}\\

\texttt{PREVIOUS FUNCTION}\\

\texttt{FEEDBACK}\\

Based on the feedback given and the function you generated previously, what are some conclusions you can draw from the feedback? Make sure to cite the specific examples in the feedback to justify your analysis.\\


Based on the feedback provided, there are several conclusions that can be drawn:\\

1. **Accuracy of the Function**: The function you generated seems to be somewhat accurate in predicting the end of game scores for the players, but there is still room for improvement. In some cases, the estimated scores match closely with the lookahead search, while in others, there is a noticeable discrepancy. For example, in Example 16, the estimated scores were quite close, but in Example 39, there was a larger difference.\\

2. **Consistency in Performance**: The function you generated seems to perform consistently across different game states. For instance, in multiple examples (e.g., Example 30, Example 40), the function consistently returned the same values for the end of game scores, even though they were not always perfectly accurate.\\

3. **Impact of Intermediate Values**: The intermediate values used in the calculation of the scores may have an impact on the accuracy of the function. In the provided feedback, there is a placeholder intermediate value 'example value' that is used in the calculation. It's possible that refining or introducing new intermediate values could improve the accuracy of the function.\\

4. **Effectiveness of Player Win Rates**: The function uses player win rates as a key factor in evaluating the state. While this is a useful approach, it may need to be refined based on the specific dynamics of The Resistance: Avalon. For example, the function currently assumes a fixed win rate for Good and Evil players, which may not capture the complexities of the game accurately.\\

Based on the function, feedback, and conclusions you drew, what are 2 improvements that you can make to the function that you think will have the most impact? Be as specific and concrete as possible, and write them out in the following format:\\
        
        
Thoughts: <your thoughts here>

Idea 1: <your idea here>

Idea 2: <your idea here>

...

Here's an example of what this might look like for 3 improvement ideas:\\

Thoughts: I should consider the number of cards left in the deck when evaluating the value of a state.

Idea 1: I should add a term to the value function that penalizes states where there are fewer cards left in the deck.

Idea 2: I should add a term to the value function that rewards states where the player has more cards in their hand than the opponent.

Idea 3: I should add a term to the value function that rewards states where the player has more cards in their hand than the opponent and there are fewer cards left in the deck.
\end{tcolorbox}
\begin{tcolorbox}[colback=white,colframe=black,title=Thoughts]
The current function relies on a simplistic win rate calculation for Good and Evil players, which may not accurately capture the dynamics of The Resistance: Avalon. Additionally, the function does not take into account the specific roles of Merlin, Assassin, Minions, and Servants, which are crucial in determining the outcome of the game.

\bigskip

\textbf{Idea 1:} Introduce role-specific win rates based on the dynamics of the roles in The Resistance: Avalon. For example, assign higher win rates to Merlin and Servants for successful quests, and lower win rates to Minions and Assassin for failed quests. This will better reflect the strategic importance of each role in achieving the objectives of their respective teams.

\bigskip

\textbf{Idea 2:} Incorporate information asymmetry between Good and Evil players into the evaluation function. For example, consider adjusting win rates based on the knowledge that Evil players have about their teammates, while Good players lack this information. This asymmetry can significantly impact the decision-making and outcomes in the game, and should be reflected in the evaluation of states.
\end{tcolorbox}


\begin{tcolorbox}[title=Avalon value heuristic idea generation output,  colframe=blue]
  Placeholder
\end{tcolorbox}

\begin{tcolorbox}[title=Avalon value heuristic strategy implementation prompt,  colframe=blue]
  Placeholder
\end{tcolorbox}

\begin{tcolorbox}[title=Avalon value heuristic strategy implementation output,  colframe=blue]
  Placeholder
\end{tcolorbox}

\begin{tcolorbox}[colback=white,colframe=black,title=Game Discussion Summary]
You are Player 0, with identity Merlin. You are on the side of Good. The Evil players are Players 2 and 4. Please do not forget your identity throughout the game. Here is a summary of previous rounds of discussion so far:

\textbf{Round 1 Discussion:}
\begin{itemize}
    \item \textbf{Player 1:} "Greetings, fellow players. As a Servant of Arthur, my primary goal is to ensure the success of our Quests. I am committed to working together with all of you to achieve victory for Good..."
    \item \textbf{Player 2:} "Greetings, noble companions. I echo Player 1's sentiment in working together for the success of our Quests..."
    \item \textbf{Player 3:} "Greetings, noble companions. I echo the sentiments shared by Player 1 and Player 2 regarding our shared goal of ensuring the success of our Quests..."
    \item \textbf{Player 4:} "Greetings, honorable players. I appreciate the dedication and commitment displayed by Player 1, Player 2, and Player 3 towards our common goal of ensuring the success of this Quest..."
\end{itemize}

\textbf{Round 2 Discussion:}
\begin{itemize}
    \item \textbf{Player 1:} "Greetings, fellow players. As a Servant of Arthur, my primary goal is to ensure the success of our Quests. I am committed to working together with all of you to achieve victory for Good..."
    \item \textbf{Player 2:} "Greetings, noble companions. I echo Player 1's sentiment in working together for the success of our Quests..."
    \item \textbf{Player 3:} "Greetings, noble companions. I echo the sentiments shared by Player 1 and Player 2 regarding our shared goal of ensuring the success of our Quests..."
    \item \textbf{Player 4:} "Greetings, honorable players. I appreciate the dedication and commitment displayed by Player 1, Player 2, and Player 3 towards our common goal of ensuring the success of this Quest..."
\end{itemize}
\end{tcolorbox}

\subsection{Avalon Dialogue Guide}
\begin{tcolorbox}[title=Avalon dialogue guide idea generation prompt,  colframe=blue]
  Placeholder
\end{tcolorbox}

\begin{tcolorbox}[title=Avalon dialogue guide idea generation output,  colframe=blue]
  Placeholder
\end{tcolorbox}

\begin{tcolorbox}[title=Avalon dialogue guide strategy implementation prompt,  colframe=blue]
  Placeholder
\end{tcolorbox}

\begin{tcolorbox}[title=Avalon dialogue guide strategy implementation output,  colframe=blue]
  Placeholder
\end{tcolorbox}




\section{Example generated strategies and improvement ideas}
\subsection{GOPS Value Heuristic}




\subsection{Avalon Value Heuristic}

\subsubsection{Idea generation}

\begin{tcolorbox}[title=Feedback thought prompt, breakable,colback=white,colframe=black]
Below is some feedback on how the function you generated performed when we tested it. Note that simulations involve high variance and the actual scores may not match the expected scores exactly. Hence, you should focus on trying to get the scores produced by your function to match those predicted by look-ahead search as closely as possible. \\

Feedback: \\

    ---
    Example 19: \\
    The state you were trying to estimate a value for is: \\
    State((3, 1, 1, 1, False, (2, 3, 4), (0, 0, 1, 1, 0, 1), (1, 1), (True,), (5, 5, 5, 0, 6, 7), (2, 3, 4, 5), ((0, 0), (1, 0))), {}) \\

    The function you generated returned the following values: \\
    \{0: 1.0, 1: 1.0, 2: 1.0, 3: 1.0, 4: -1.0, 5: -1.0\} \\
    for the expected end of game scores of the players. \\

    Some intermediate values that you used to calculate the scores were: \\
    \{'num_successful_quests': 1, 'num_failed_quests': 0\} \\

    The estimated end of game scores of the players using lookahead search with your function was: \\
    \{0: 0.9999999754633906, 1: 0.9999999754633906, 2: 0.9999999754633906, 3: 0.9999999754633906, 4: -0.9999999754633906, 5: -0.9999999754633906\} \\

    The actual scores of the players at the end of the game in the simulation were: \\
    \{0: -1.0, 1: -1.0, 2: -1.0, 3: -1.0, 4: 1.0, 5: 1.0\} \\
    --- \\
        
Based on the feedback given and the function you generated previously, what are some conclusions you can draw from the feedback? Make sure to cite the specific examples in the feedback to justify your analysis.\\
\end{tcolorbox}


\begin{tcolorbox}[title=Feedback thought response, breakable,colback=white,colframe=blue]
Based on the feedback provided, it is evident that the function I generated to evaluate the value of a state in The Resistance: Avalon game is not accurately predicting the end-game scores of the players. The expected end of game scores returned by the function do not match the actual scores observed in the simulations, as shown in the examples provided.\\

Specifically, in Example 11, the function returned expected end of game scores of \{0: 1.0, 1: 1.0, 2: -1.0, 3: 1.0, 4: 1.0, 5: -1.0\}, while the actual scores were \{0: -1.0, 1: -1.0, 2: 1.0, 3: -1.0, 4: -1.0, 5: 1.0\}. This discrepancy is also observed in other examples provided in the feedback.\\

The function seems to oversimplify the evaluation of player win rates based on the number of successful and failed quests, without taking into account the strategic interactions and hidden information involved in the game. As a result, the function's predictions do not align with the outcomes of the actual game simulations.\\

In conclusion, the function I generated needs to be improved to better capture the complexities of The Resistance: Avalon game, such as hidden roles, player deception, and strategic decision-making. It is important to consider the unique dynamics of the game in order to develop a more accurate value heuristic for evaluating game states.
\end{tcolorbox}

\begin{tcolorbox}[title=Idea generation prompt, breakable,colback=white,colframe=black]
Based on the function, feedback, and conclusions you drew, what are 2 improvements that you can make to the function that you think will have the most impact? Be as specific and concrete as possible, mentioning specific code pieces or helper functions that you can add. If the game has different phases, you can also mention what specific phase the idea applies to. Write them out in the following format:\\

Thoughts: \\
<your thoughts here>\\

Idea 1: \\
<your idea here>\\

Idea 2: \\
<your idea here>\\


Here's an example of what this might look like for 3 improvement ideas:\\

Thoughts: \\
The feedback suggests that the main problem is that function is not taking into account the cards in either player's hand, which leads to inaccurate value estimates.\\

Idea 1: \\
I can calculate the difference in the number of cards in each player's hand, increasing the estimated value of players with more cards in their hand.\\

Idea 2: \\
I can write a helper function that compares the sum of the values of the cards in each player's hand, increasing the estimated value of players with higher total card values.\\

Idea 3: \\
During the draw phase, I can also calculate the expected values of the cards that the players will draw, increasing the estimated value of players with higher expected card values.
\end{tcolorbox}

\begin{tcolorbox}[title=Idea generation response, breakable,colback=white,colframe=blue]
Thoughts: \\
The feedback indicates that the current function is oversimplifying the evaluation of player win rates based on the number of successful and failed quests, without considering the strategic interactions and hidden information in the game. To improve the accuracy of the function, we need to incorporate these elements into the heuristic.\\

Idea 1: \\
Introduce a role-aware win rate calculation by taking into account the specific roles assigned to each player. For example, Merlin and Assassin have critical roles that can heavily influence the outcome of the game. We can modify the function to assign different weights to the win rates of players based on their roles. This can be achieved by creating a dictionary that maps each role to a specific win rate multiplier, and then adjusting the win rates of players accordingly based on their roles.\\

Idea 2: \\
Implement a strategic depth factor that accounts for the impact of strategic decisions made by players during the game. This can involve analyzing the voting patterns, quest selections, and other strategic moves to determine how they affect the overall outcome. By incorporating a strategic depth factor into the function, we can provide a more nuanced evaluation of the state based on the strategic decisions made by players. This can be done by introducing a new parameter in the function that represents the strategic depth factor, which adjusts the win rates of players based on the strategic complexity of the game state.
\end{tcolorbox}


\subsubsection{Strategy implementation}

% \begin{tcolorbox}[title=Avalon Value Heuristics Function (Before)]
% \begin{lstlisting}[language=Python, breaklines=true]
% def evaluate_state(state):
%     # Extract information from the game state
%     players = state['players']
%     historical_quest_results = state['historical_quest_results']
%     is_good = state['is_good']

%     # Initialize win rate dictionary and intermediate values dictionary
%     expected_winrates_per_player = {}
%     intermediate_values = {}
    
%     # Calculate the number of successful and failed quests
%     num_successful_quests = sum(historical_quest_results)
%     num_failed_quests = len(historical_quest_results) - num_successful_quests
    
%     # Store the number of successful and failed quests in the intermediate values dictionary
%     intermediate_values['num_successful_quests'] = num_successful_quests
%     intermediate_values['num_failed_quests'] = num_failed_quests
    
%     # Calculate the total number of quests
%     total_quests = len(historical_quest_results)
    
%     # Avoid division by zero error by checking if total_quests is zero
%     if total_quests == 0:
%         for player in players:
%             expected_winrates_per_player[player] = 0.5 # Assign each player a win rate of 0.5 if no quests have been attempted yet
%     else:
%         # Calculate the win rates for each player
%         for player in players:
%             if is_good[player]:
%                 # The win rate for a good player is equal to the number of successful quests 
%                 # divided by the total number of quests
%                 expected_winrates_per_player[player] = num_successful_quests / total_quests
%             else:
%                 # The win rate for an evil player is equal to the number of failed quests 
%                 # divided by the total number of quests
%                 expected_winrates_per_player[player] = num_failed_quests / total_quests

%     return expected_winrates_per_player, intermediate_values
% \end{lstlisting}
% \end{tcolorbox}








\begin{tcolorbox}[title=Best value heuristic for Avalon]
  Placeholder
\end{tcolorbox}

\begin{tcolorbox}[title=Best improvement idea for Avalon value function]
  Placeholder
\end{tcolorbox}

\subsection{Avalon Dialogue Guide}
\begin{tcolorbox}[title=Best dialogue guide for Avalon]
  Placeholder
\end{tcolorbox}

\begin{tcolorbox}[title=Best improvement idea for Avalon dialogue guide]
  Placeholder
\end{tcolorbox}

\section{Example strategy improvements}

\begin{tcolorbox}[title=Best improvement idea for Avalon dialogue guide]
  Placeholder
\end{tcolorbox}

\begin{tcolorbox}[title=Best improvement idea for Avalon dialogue guide]
  Placeholder
\end{tcolorbox}

\begin{tcolorbox}[title=Best improvement idea for Avalon dialogue guide]
  Placeholder
\end{tcolorbox}
